# Supplementary material for: Bayesian inference on the number of recurrent events: A joint model of recurrence and survival
Source: arXiv:2005.06819 source file (2021-08-03)
Supplement: Supplementary file 1 [file supp_web.pdf]

# Supplemental material for “Bayesian inference on the number of recurrent events: A joint model of recurrence and survival” by Willem van den Boom, Maria De Iorio and Marta Tallarita

## S1 Gibbs sampler

This appendix describes the Gibbs sampler summarized in Algorithm S1.

### S1.1 Normalization constant in $p(\boldsymbol{Y}_i, S_i \mid \text{—})$

The distribution $p(\boldsymbol{Y}_i, S_i \mid \text{—})$ defined in (2) is truncated by $T_{iN_i} \leq S_i$. Thus, the normalization constant of $p(\boldsymbol{Y}_i, S_i \mid \text{—})$ depends on parameters of interest and is thus required to be able to

---

**Algorithm S1** Gibbs sampler

---

For each iteration of the Gibbs sampler:

1. For $k = 1, \ldots, q$, update $\beta_k$ and $\gamma_k$ by slice sampling with (S6) and (S9).
2. For each censored individual $i$:
   (a) Update $N_i$ and $Y_{i(n_i+1)}^{N_i}$ using the reversible jump sampler from Section S1.3.
   (b) For $j = n_i + 1, \ldots, N_i$, sample $Y_{ij}$ from (S10) truncated by $T_{i(n_i+1)} > c_i$ and $T_{iN_i} \leq S_i$ using the inverse transformation method.
   (c) Sample $S_i$ from (S7) truncated by $S_i > \max(c_i, T_{iN_i})$ using the inverse transformation method.
3. Update $\boldsymbol{m}_i$ and $\delta_i$ for $i = 1, \ldots, L$ via Algorithm 8 from Neal (2000) using slice sampling with (S11–S13).
4. Sample $M$ from the distribution in Equation 13 from Escobar and West (1995).
5. Update $\sigma^2$, $\eta^2$, $r$ and $\lambda$ by slice sampling with (S14–S16).

---

sample from the full conditionals of these parameters. This differs from previous likelihood specifications with log-normally distributed gap times (Aalen and Husebye, 1991; Paulon et al., 2018; Tallarita et al., 2020) because $p(\boldsymbol{Y}_i \mid \boldsymbol{\beta}, \boldsymbol{m}_i, N_i, S_i, \sigma^2, \boldsymbol{x}_i)$ is conditional on the number of events $N_i$.

To derive the normalization constant of $p(\boldsymbol{Y}_i, S_i \mid —)$, note that by (3)

$$f(\boldsymbol{Y}_i \mid \boldsymbol{\beta}, \boldsymbol{m}_i, N_i, \sigma^2, \boldsymbol{x}_i) = \mathcal{N}_{N_i}(\boldsymbol{Y}_i \mid \boldsymbol{\mu}_{\boldsymbol{Y}_i},\, \boldsymbol{\Sigma}_{\boldsymbol{Y}_i}), \tag{S1}$$

where $\boldsymbol{\mu}_{\boldsymbol{Y}_i} = (\boldsymbol{x}_i^T\boldsymbol{\beta} + m_{i1})\,\mathbf{1}_{N_i\times 1}$ and the $N_i \times N_i$ matrix $\boldsymbol{\Sigma}_{\boldsymbol{Y}_i}$ is defined by its tridiagonal inverse $\boldsymbol{\Sigma}_{\boldsymbol{Y}_i}^{-1}$ with $(\boldsymbol{\Sigma}_{\boldsymbol{Y}_i}^{-1})_{jj} = (m_{i2}^2 + 1)/\sigma^2$ for $j = 1, \ldots, N_i - 1$, $(\boldsymbol{\Sigma}_{\boldsymbol{Y}_i}^{-1})_{N_iN_i} = 1/\sigma^2$ and $(\boldsymbol{\Sigma}_{\boldsymbol{Y}_i}^{-1})_{j_1j_2} = -m_{i2}/\sigma^2$ for $|j_1 - j_2| = 1$.[1] Consider now the untruncated $\boldsymbol{Y}_i^* \sim \mathcal{N}_{N_i}(\boldsymbol{\mu}_{\boldsymbol{Y}_i},\, \boldsymbol{\Sigma}_{\boldsymbol{Y}_i})$ and define $T_{iN_i}^* = \sum_{j=1}^{N_i} e^{Y_{ij}^*}$. Similarly, define an untruncated and independent $S_i^*$ by

$$\log(S_i^*) \sim \mathcal{N}\left\{\boldsymbol{x}_i^T\boldsymbol{\gamma} + \delta_i,\, \eta^2\right\} \tag{S2}$$

based on (4). Then, the normalization constant of $p(\boldsymbol{Y}_i, S_i \mid —)$ equals $\Pr(T_{iN_i}^* \leq S_i^*)$ where we drop the conditioning on $\boldsymbol{\beta}$, $\boldsymbol{\gamma}$, $\boldsymbol{m}_i$, $\delta_i$, $N_i$, $\sigma^2$ and $\eta^2$ for notational convenience. For $N_i = 0$, $T_{iN_i}^* = T_{i0}^* = 0$ such that $\Pr(T_{iN_i}^* \leq S_i^*) = 1$. Therefore, the remainder of this subsection considers only $N_i \geq 1$. $T_{iN_i}^*$ is the sum of log-normal random variables. The distribution of such sums and $\Pr(T_{iN_i}^* \leq S_i^*)$ have no closed-form expression (Asmussen et al., 2019), requiring us to resort to approximations.

It is infeasible to evaluate $\Pr(T_{iN_i}^* \leq S_i^*)$ by numerical integration using quadrature for the values of $N_i$ that we encounter. Fortunately, there is a literature on approximating $\Pr(T_{iN_i}^* \leq s)$ for fixed $s$ (Botev et al., 2019, and references therein) which includes deterministic and Monte Carlo methods. As we aim to sample from the full conditionals of $\boldsymbol{\beta}$, $\boldsymbol{\gamma}$, $\boldsymbol{m}_i$, $\delta_i$, $N_i$, $\sigma^2$ and $\eta^2$ as part of a Gibbs sampler, we need to evaluate the normalization constant $\Pr(T_{iN_i}^* \leq S_i^*)$ many times, requiring a fast approximation. We therefore choose the Fenton-Wilkinson method (Fenton, 1960) which approximates the distribution of $T_{iN_i}^*$ by a log-normal distribution with matched mean and variance. Asmussen et al. (2019) state that this approximation can be inaccurate for small $N_i$ and when the elements in $\boldsymbol{Y}_i^*$ are dependent. However, their numerical results indicate good performance of the Fenton-Wilkinson method under these circumstances. Other fast approximations such as the saddle-point method from Asmussen et al. (2016) might be much more accurate, though they are also more complex than the Fenton-Wilkinson method.

For any matrix $\boldsymbol{A}$, denote the elementwise exponential by $e^{\boldsymbol{A}}$. Define $\text{diag}(\boldsymbol{\Sigma}_{\boldsymbol{Y}_i}) = \{(\boldsymbol{\Sigma}_{\boldsymbol{Y}_i})_{11}, \ldots, (\boldsymbol{\Sigma}_{\boldsymbol{Y}_i})_{N_iN_i}\}^T$. For any vector $\boldsymbol{a}$, denote the outer product with itself by $\boldsymbol{a}^{2\otimes} = \boldsymbol{a}\boldsymbol{a}^T$. Then,

$$\begin{aligned}
\text{E}(e^{\boldsymbol{Y}_i^*}) &= e^{\boldsymbol{\mu}_{\boldsymbol{Y}_i} + \text{diag}(\boldsymbol{\Sigma}_{\boldsymbol{Y}_i})/2} &&= e^{\boldsymbol{x}_i^T\boldsymbol{\beta} + m_{i1}}\, e^{\text{diag}(\boldsymbol{\Sigma}_{\boldsymbol{Y}_i})/2},\\
\text{Cov}(e^{\boldsymbol{Y}_i^*}) &= \text{E}(e^{\boldsymbol{Y}_i^*})^{2\otimes} \circ (e^{\boldsymbol{\Sigma}_{\boldsymbol{Y}_i}} - \mathbf{1}_{N_i\times N_i}) &&= e^{2(\boldsymbol{x}_i^T\boldsymbol{\beta} + m_{i1})} \left\{e^{\text{diag}(\boldsymbol{\Sigma}_{\boldsymbol{Y}_i})/2}\right\}^{2\otimes} \circ (e^{\boldsymbol{\Sigma}_{\boldsymbol{Y}_i}} - \mathbf{1}_{N_i\times N_i});
\end{aligned}$$

[1]This implies $(\boldsymbol{\Sigma}_{\boldsymbol{Y}_i})_{j_1j_2} = (m_{i2}^{|j_1-j_2|} - m_{i2}^{j_1+j_2})/(1 - m_{i2}^2)$ for $j_1, j_2 = 1, \ldots, N_i$.

where '$\circ$' denotes the Hadamard product (Halliwell, 2015). Since $T^*_{iN_i} = \mathbf{1}_{1\times N_i}\, e^{\boldsymbol{Y}_i^*}$,

$$\begin{aligned}
\mathrm{E}(T^*_{iN_i}) &= \mathbf{1}_{1\times N_i}\ \mathrm{E}(e^{\boldsymbol{Y}_i^*}) = e^{\boldsymbol{x}_i^T\boldsymbol{\beta}+m_{i1}}\ \mathrm{sum}\{e^{\mathrm{diag}(\boldsymbol{\Sigma}_{\boldsymbol{Y}_i})/2}\},\\
\mathrm{Var}(T^*_{iN_i}) &= \mathbf{1}_{1\times N_i}\ \mathrm{Cov}(e^{\boldsymbol{Y}_i^*})\,\mathbf{1}_{N_i\times 1} \qquad \text{(S3)}\\
&= e^{2(\boldsymbol{x}_i^T\boldsymbol{\beta}+m_{i1})}\ \mathrm{sum}[\{e^{\mathrm{diag}(\boldsymbol{\Sigma}_{\boldsymbol{Y}_i})/2}\}^{2\otimes}\circ(e^{\boldsymbol{\Sigma}_{\boldsymbol{Y}_i}} - \mathbf{1}_{N_i\times N_i})];
\end{aligned}$$

where sum($\cdot$) denotes the grand sum of a matrix which is the sum of all its elements. The Fenton-Wilkinson approximation to the distribution of $T^*_{iN_i}$ is a log-normal distribution with the same mean and variance. Let $\hat{T}^*_{iN_i}$ be distributed according to this log-normal distribution. Then, $\log(\hat{T}^*_{iN_i}) \sim \mathcal{N}[\log\{\mathrm{E}(T^*_{iN_i})\} - A,\, 2A]$ with

$$\begin{aligned}
A &= \frac{1}{2}\log\left\{1+\frac{\mathrm{Var}(T^*_{iN_i})}{\mathrm{E}(T^*_{iN_i})^2}\right\}\\
&= \frac{1}{2}\log(\mathrm{sum}[\{e^{\mathrm{diag}(\boldsymbol{\Sigma}_{\boldsymbol{Y}_i})/2}\}^{2\otimes}\circ e^{\boldsymbol{\Sigma}_{\boldsymbol{Y}_i}}]) - \log[\mathrm{sum}\{e^{\mathrm{diag}(\boldsymbol{\Sigma}_{\boldsymbol{Y}_i})/2}\}]\\
&= \frac{\mathrm{LS}_2}{2} - \mathrm{LS}_1,
\end{aligned}$$

where the second equality follows from (S3) and $\mathrm{sum}\{e^{\mathrm{diag}(\boldsymbol{\Sigma}_{\boldsymbol{Y}_i})/2}\}^2 = \mathrm{sum}[\{e^{\mathrm{diag}(\boldsymbol{\Sigma}_{\boldsymbol{Y}_i})/2}\}^{2\otimes}]$, and $\mathrm{LS}_1 = \log[\mathrm{sum}\{e^{\mathrm{diag}(\boldsymbol{\Sigma}_{\boldsymbol{Y}_i})/2}\}]$ and $\mathrm{LS}_2 = \log(\mathrm{sum}[\{e^{\mathrm{diag}(\boldsymbol{\Sigma}_{\boldsymbol{Y}_i})/2}\}^{2\otimes}\circ e^{\boldsymbol{\Sigma}_{\boldsymbol{Y}_i}}])$ are introduced for notational convenience. Moreover, by standard properties of the Gaussian distribution, the independence of $\hat{T}^*_{iN_i}$ and $S^*_i$ and (S2),

$$\log(\hat{T}^*_{iN_i}) - \log(S^*_i) \sim \mathcal{N}[\log\{\mathrm{E}(T^*_{iN_i})\} - A - \boldsymbol{x}_i^T\boldsymbol{\gamma} - \delta_i,\, 2A+\eta^2].$$

Our approximation to the normalization constant is thus

$$\begin{aligned}
\Pr(T^*_{iN_i}\le S^*_i) &\approx \Pr\{\hat{T}^*_{iN_i}\le S^*_i\} = \Pr\{\log(\hat{T}^*_{iN_i}) - \log(S^*_i)\le 0\}\\
&= \Phi\left[\frac{-\log\{\mathrm{E}(T^*_{iN_i})\} + A + \boldsymbol{x}_i^T\boldsymbol{\gamma} + \delta_i}{\sqrt{2A+\eta^2}}\right]\\
&= \Phi\left\{\frac{-\boldsymbol{x}_i^T\boldsymbol{\beta} - m_{i1} - 2\,\mathrm{LS}_1 + \mathrm{LS}_2/2 + \boldsymbol{x}_i^T\boldsymbol{\gamma} + \delta_i}{\sqrt{\mathrm{LS}_2 - 2\,\mathrm{LS}_1 + \eta^2}}\right\},
\end{aligned}$$

where $\Phi(\cdot)$ is the cumulative density function of $\mathcal{N}(0,\,1)$ and the last equality follows from (S3). In the remainder of this appendix, we write $\Pr(T^*_{iN_i}\le S^*_i)$ even though we use this approximation.

$\mathrm{LS}_1$ and $\mathrm{LS}_2$ only depend on $\boldsymbol{\Sigma}_{\boldsymbol{Y}_i}$. Therefore, we only need to recompute $\mathrm{LS}_1$ and $\mathrm{LS}_2$ in the Gibbs sampler when $\boldsymbol{\Sigma}_{\boldsymbol{Y}_i}$, which is a function of $m_{i2}$, $\sigma^2$ and $N_i$, changes.

## S1.2 Regression coefficients

The full conditional for $\boldsymbol{\beta}$ follows from the prior and the likelihood in Section 2.2 as

$$p(\boldsymbol{\beta}\mid -) \propto \mathcal{N}_q(\boldsymbol{\beta}\mid 0,\, \sigma^2_\beta \boldsymbol{I}_q)\prod_{i=1}^{L} p(\boldsymbol{Y}_i, S_i\mid -). \qquad \text{(S4)}$$

We can use the expression for $f(\boldsymbol{Y}_i \mid \boldsymbol{\beta}, \boldsymbol{m}_i, N_i, \sigma^2, \boldsymbol{x}_i)$ in (3) or (S1) directly to evaluate (S4), but that is computationally expensive as it involves a multitude of Gaussian density evaluations. Instead, we introduce $Y_{i1}^{\boldsymbol{\beta}} = Y_{i1} - m_{i1}$, $Y_{ij}^{\boldsymbol{\beta}} = \{Y_{ij} - m_{i1} - m_{i2}(Y_{i(j-1)} - m_{i1})\}/(1 - m_{i2})$ for $j = 2, \ldots, N_i$ and the $N_i \times N_i$ diagonal matrix $\boldsymbol{\Sigma}_{\boldsymbol{\beta},i}$ with $\text{diag}(\boldsymbol{\Sigma}_{\boldsymbol{\beta},i}) = \sigma^2 \{1, (1 - m_{i2})^{-2}, \ldots, (1 - m_{i2})^{-2}\}^T$. Then, we can rewrite (3) as

$$f(\boldsymbol{Y}_i \mid \boldsymbol{\beta}, \boldsymbol{m}_i, N_i, \sigma^2, \boldsymbol{x}_i) = \mathcal{N}_{N_i}(\boldsymbol{Y}_i^{\boldsymbol{\beta}} \mid \mathbf{1}_{N_i \times 1}\, \boldsymbol{x}_i^T \boldsymbol{\beta},\, \boldsymbol{\Sigma}_{\boldsymbol{\beta},i}), \quad T_{iN_i} \leq S_i.$$

Inserting this expression into (S4) yields a normal-normal model such that

$$p(\boldsymbol{\beta} \mid -) \propto \frac{\mathcal{N}_q(\boldsymbol{\beta} \mid \boldsymbol{\mu}_{\boldsymbol{\beta}}^*,\, \boldsymbol{\Sigma}_{\boldsymbol{\beta}}^*)}{\prod_{i=1}^L \Pr(T_{iN_i}^* \leq S_i^*)}, \tag{S5}$$

where $\boldsymbol{\mu}_{\boldsymbol{\beta}}^* = \boldsymbol{\Sigma}_{\boldsymbol{\beta}}^* \sum_{i=1}^L \boldsymbol{x}_i \mathbf{1}_{1 \times N_i} \boldsymbol{\Sigma}_{\boldsymbol{\beta},i}^{-1} \boldsymbol{Y}_i^{\boldsymbol{\beta}}$, and $\boldsymbol{\Sigma}_{\boldsymbol{\beta}}^* = \{\boldsymbol{I}_q/\sigma_\beta^2 + \sum_{i=1}^L \text{sum}(\boldsymbol{\Sigma}_{\boldsymbol{\beta},i}^{-1})\, \boldsymbol{x}_i \boldsymbol{x}_i^T\}^{-1}$ with $\text{sum}(\boldsymbol{\Sigma}_{\boldsymbol{\beta},i}^{-1}) = \{1 + (N_i - 1)(1 - m_{i2})^2\}/\sigma^2$ for $N_i \geq 1$ and $\text{sum}(\boldsymbol{\Sigma}_{\boldsymbol{\beta},i}^{-1}) = 0$ for $N_i = 0$. Recalling the conditional distributions of a multivariate normal, we obtain

$$p(\beta_k \mid -) \propto \frac{\mathcal{N}(\beta_k \mid \mu_{\beta_k}^*,\, \Sigma_{\beta_k}^*)}{\prod_{i=1}^L \Pr(T_{iN_i}^* \leq S_i^*)}, \tag{S6}$$

where $\mu_{\beta_k}^* = (\boldsymbol{\mu}_{\boldsymbol{\beta}}^*)_k + (\boldsymbol{\Sigma}_{\boldsymbol{\beta}}^*)_{k,-k} (\boldsymbol{\Sigma}_{\boldsymbol{\beta}}^*)_{-k,-k}^{-1} \{\boldsymbol{\beta}_{-k} - (\boldsymbol{\mu}_{\boldsymbol{\beta}}^*)_{-k}\}$ and
$\Sigma_{\beta_k}^* = (\boldsymbol{\Sigma}_{\boldsymbol{\beta}}^*)_{kk} - (\boldsymbol{\Sigma}_{\boldsymbol{\beta}}^*)_{k,-k} (\boldsymbol{\Sigma}_{\boldsymbol{\beta}}^*)_{-k,-k}^{-1} (\boldsymbol{\Sigma}_{\boldsymbol{\beta}}^*)_{k,-k}^T$ with the $1 \times (q-1)$ row vector $(\boldsymbol{\Sigma}_{\boldsymbol{\beta}}^*)_{k,-k}$ equal to the $k$th row of $\boldsymbol{\Sigma}_{\boldsymbol{\beta}}^*$ without its $k$th element, the $(q-1) \times (q-1)$ matrix $(\boldsymbol{\Sigma}_{\boldsymbol{\beta}}^*)_{-k,-k}$ equal to $\boldsymbol{\Sigma}_{\boldsymbol{\beta}}^*$ without its $k$th row and $k$th column, and $\boldsymbol{a}_{-k}$ equal to the vector $\boldsymbol{a}$ without its $k$th element, for $k = 1, \ldots, q$. Now, the Gibbs update for $\boldsymbol{\beta}$ follows as slice sampling with (S6) as target density for $k = 1, \ldots, q$.

For the other regression coefficient $\boldsymbol{\gamma}$, consider (2) and (4) such that

$$f\{\log(S_i) \mid -\} \propto \mathcal{N}\{\log(S_i) \mid \boldsymbol{x}_i^T \boldsymbol{\gamma} + \delta_i,\, \eta^2\}, \quad S_i \geq T_{iN_i}. \tag{S7}$$

The full conditional for $\boldsymbol{\gamma}$ then follows with the prior $\boldsymbol{\gamma} \sim \mathcal{N}_q(0,\, \sigma_\gamma^2\, \boldsymbol{I}_q)$ from Section 2.3 as

$$p(\boldsymbol{\gamma} \mid -) \propto \mathcal{N}_q(\boldsymbol{\gamma} \mid 0,\, \sigma_\gamma^2\, \boldsymbol{I}_q) \prod_{i=1}^L p\{\log(S_i) \mid -\} \propto \frac{\mathcal{N}_q(\boldsymbol{\gamma} \mid \boldsymbol{\mu}_{\boldsymbol{\gamma}}^*,\, \boldsymbol{\Sigma}_{\boldsymbol{\gamma}}^*)}{\prod_{i=1}^L \Pr(T_{iN_i}^* \leq S_i^*)} \tag{S8}$$

where $\boldsymbol{\mu}_{\boldsymbol{\gamma}}^* = \boldsymbol{\Sigma}_{\boldsymbol{\gamma}}^* \boldsymbol{X}^T (\boldsymbol{U} - \boldsymbol{\delta})/\eta^2$ and $\boldsymbol{\Sigma}_{\boldsymbol{\gamma}}^* = (\boldsymbol{I}_q/\sigma_\gamma^2 + \boldsymbol{X}^T \boldsymbol{X}/\eta^2)^{-1}$ with the $L \times q$ matrix $\boldsymbol{X} = (\boldsymbol{x}_1, \ldots, \boldsymbol{x}_L)^T$ and the $L$-dimensional vector $\boldsymbol{U} = \{\log(S_1), \ldots, \log(S_L)\}^T$. Analogously to (S6), we obtain

$$p(\gamma_k \mid -) \propto \frac{\mathcal{N}(\gamma_k \mid \mu_{\gamma_k}^*,\, \Sigma_{\gamma_k}^*)}{\prod_{i=1}^L \Pr(T_{iN_i}^* \leq S_i^*)}, \tag{S9}$$

where $\mu_{\gamma_k}^* = (\boldsymbol{\mu}_{\boldsymbol{\gamma}}^*)_k + (\boldsymbol{\Sigma}_{\boldsymbol{\gamma}}^*)_{k,-k} (\boldsymbol{\Sigma}_{\boldsymbol{\gamma}}^*)_{-k,-k}^{-1} \{\boldsymbol{\gamma}_{-k} - (\boldsymbol{\mu}_{\boldsymbol{\gamma}}^*)_{-k}\}$ and
$\Sigma_{\gamma_k}^* = (\boldsymbol{\Sigma}_{\boldsymbol{\gamma}}^*)_{kk} - (\boldsymbol{\Sigma}_{\boldsymbol{\gamma}}^*)_{k,-k} (\boldsymbol{\Sigma}_{\boldsymbol{\gamma}}^*)_{-k,-k}^{-1} (\boldsymbol{\Sigma}_{\boldsymbol{\gamma}}^*)_{k,-k}^T$. Similarly to $\boldsymbol{\beta}$, the Gibbs update for $\boldsymbol{\gamma}$ follows as slice sampling with (S9) as target density for $k = 1, \ldots, q$.

## S1.3 Reversible jump sampler for $N_i$

If individual $i$ is censored, then the number of events $N_i$ is unknown and object of inference. Since $N_i$ affects the dimensionality of $\boldsymbol{Y}_i$, we use a reversible jump sampler (Green, 1995; Waagepetersen and Sorensen, 2001) to update it. The sampler updates $N_i$ and $Y_{i(n_i+1)}^{N_i} = (Y_{i(n_i+1)}, \ldots, Y_{iN_i})^T$ jointly. It is a Metropolis-Hastings algorithm on a state space of varying dimension. The state space is $\bigcup_{N_i=n_i}^{\infty} \mathbb{R}^{N_i-n_i}$ in our case.

The proposal distribution for $N_i$ and $Y_{i(n_i+1)}^{N_i}$ is as follows. Since $N_i \geq n_i$, we sample $N_i \sim \mathbb{1}_{[n_i,\infty)} \operatorname{NegBin}(r, \lambda)$, a negative binomial truncated to $[n_i, \infty)$, using the inverse transformation method. To complete the joint proposal, we only need to specify the proposal distribution of $Y_{i(n_i+1)}^{N_i}$ given $N_i$. We use $T_{i(n_i+1)} \sim \mathcal{U}(c_i, S_i)$ and $T_{ij} \mid T_{i(j-1)} \sim \mathcal{U}(T_{i(j-1)}, S_i)$ for $j = n_i + 2, \ldots, N_i$ as $T_{iN_i} \leq S_i$. We prefer this proposal over sampling along the lines of (3) as then the proposal density would involve an intractable normalization constant similarly to (2). Instead, we now have $\Pr(T_{i(n_i+1)} \leq t) = (t - c_i)/(S_i - c_i)$ and $\Pr(T_{ij} \leq t \mid T_{i(j-1)}) = (t - T_{i(j-1)})/(S_i - T_{i(j-1)})$ for $j = n_i + 2, \ldots, N_i$. Inserting (1) shows $\Pr(Y_{i(n_i+1)} \leq y) = (e^y + T_{in_i} - c_i)/(S_i - c_i)$ and $\Pr(Y_{ij} \leq y \mid T_{i(j-1)}) = e^y/(S_i - T_{i(j-1)})$ for $j = n_i + 2, \ldots, N_i$. The proposal density is thus

$$f_{N_i}(Y_{i(n_i+1)}^{N_i}) = \begin{cases} \frac{e^{Y_{i(n_i+1)}+T_{n_i}-c_i}}{S_i-c_i} \prod_{j=n_i+2}^{N_i} \frac{e^{Y_{ij}}}{S_i-T_{i(j-1)}}, & N_i > n_i \\ 1, & N_i = n_i \end{cases}.$$

To derive the acceptance probability, we follow the notation in Waagepetersen and Sorensen (2001, Section 4) where proposed values are denoted by a prime ('). Specifically, the proposal distributions are written as $p_{N_iN_i'} \propto \mathbb{1}[N_i' \geq n_i] \operatorname{NegBin}(N_i' \mid r, \lambda)$ and $q_{N_iN_i'}(Y_{i(n_i+1)}^{N_i}, \cdot) = f_{N_i'}(\cdot)$. The target density follows from Sections 2.1, 2.2 and S1.1 as

$$\pi(N_i, Y_{i(n_i+1)}^{N_i}) \propto \operatorname{NegBin}(N_i \mid r, \lambda) \times \begin{cases} 1, & N_i = 0 \\ \frac{f(\boldsymbol{Y}_i \mid \boldsymbol{\beta}, \boldsymbol{m}_i, N_i, \sigma^2, \boldsymbol{x}_i)}{\Pr(T_{iN_i}^* \leq S_i^*)}, & N_i \geq 1 \end{cases}$$

for $N_i \geq n_i$, $T_{i(n_i+1)} > c_i$ and $T_{iN_i} \leq S_i$, and where $f(\boldsymbol{Y}_i \mid \boldsymbol{\beta}, \boldsymbol{m}_i, N_i, \sigma^2, \boldsymbol{x}_i)$ is given by (3). The dimension changing map can be written in the notation of Waagepetersen and Sorensen (2001, Section 4) as

$$g_{N_iN_i'}\{Y_{i(n_i+1)}^{N_i}, (Y')_{i(n_i+1)}^{N_i'}\} = \begin{pmatrix} g_{1N_iN_i'}\{Y_{i(n_i+1)}^{N_i}, (Y')_{i(n_i+1)}^{N_i'}\} \\ g_{2N_iN_i'}\{Y_{i(n_i+1)}^{N_i}, (Y')_{i(n_i+1)}^{N_i'}\} \end{pmatrix},$$

where $g_{1N_iN_i'}\{Y_{i(n_i+1)}^{N_i}, (Y')_{i(n_i+1)}^{N_i'}\} = (Y')_{i(n_i+1)}^{N_i'}$ and $g_{2N_iN_i'}\{Y_{i(n_i+1)}^{N_i}, (Y')_{i(n_i+1)}^{N_i'}\} = Y_{i(n_i+1)}^{N_i}$. The acceptance probability is then given by (Waagepetersen and Sorensen, 2001, Equation 19)

$$\begin{aligned} &a_{N_iN_i'}\{Y_{i(n_i+1)}^{N_i}, (Y')_{i(n_i+1)}^{N_i'}\} \\ &\qquad = \min\left[1, \frac{\pi\{N_i', (Y')_{i(n_i+1)}^{N_i'}\}\, p_{N_i'N_i}\, q_{N_i'N_i}\{(Y')_{i(n_i+1)}^{N_i'}, Y_{i(n_i+1)}^{N_i}\}}{\pi(N_i, Y_{i(n_i+1)}^{N_i})\, p_{N_iN_i'}\, q_{N_iN_i'}\{Y_{i(n_i+1)}^{N_i}, (Y')_{i(n_i+1)}^{N_i'}\}} \left|J_{g_{N_iN_i'}}\right|\right], \end{aligned}$$

where $|J_{g_{N_i N_i'}}|$ denotes the absolute value of the determinant of the Jacobian of $g_{N_i N_i'}$. The elements of $J_{g_{N_i N_i'}}$ are all zero except for one entry in each row that equals one so that the absolute value of its determinant equals one. Additionally substituting the definitions of the various terms yields as acceptance probability

$$a_{N_i N_i'}\{Y_{i(n_i+1)}^{N_i}, (Y')_{i(n_i+1)}^{N_i'}\} = \min\left[1,\ \frac{C_{N_i'}\{(Y')_{i(n_i+1)}^{N_i'}\}}{C_{N_i}(Y_{i(n_i+1)}^{N_i})} \times \frac{f_{N_i}(Y_{i(n_i+1)}^{N_i})}{f_{N_i'}\{(Y')_{i(n_i+1)}^{N_i'}\}}\right],$$

where

$$C_{N_i}(Y_{i(n_i+1)}^{N_i}) = \begin{cases} 1, & N_i = 0 \\ \frac{f(\boldsymbol{Y}_i|\boldsymbol{\beta},\boldsymbol{m}_i,N_i,\sigma^2,\boldsymbol{x}_i)}{\Pr(T_{iN_i}^* \le S_i^*)}, & N_i \ge 1 \end{cases}.$$

This reversible jump sampler updates both $N_i$ and $Y_{i(n_i+1)}^{N_i}$. Additionally, we update $Y_{i(n_i+1)}^{N_i}$ as described in the next section to improve mixing of the Gibbs sampler in case the Metropolis-Hastings sampler in this section rarely accepts the proposed samples.

## S1.4 Survival and log gap times

If individual $i$ is censored, then the log gap times $Y_{i(n_i+1)}^{N_i}$ and the survival time $S_i$ are imputed in the Gibbs sampler. The full conditional for the vector $Y_{i(n_i+1)}^{N_i}$ is hard to sample from due to the truncation $T_{iN_i} \le S_i$. Instead, we consider its elementwise full conditionals. By (2) and (3), for $j = 2, \dots, N_i - 1$,

$$\begin{aligned} p(Y_{i1} \mid \text{—}) &\propto \begin{cases} \mathcal{N}(Y_{i1} \mid \boldsymbol{x}_i^T\boldsymbol{\beta} + m_{i1},\, \sigma^2), & N_i = 1, \\ \mathcal{N}\left\{Y_{i1} \;\middle|\; \boldsymbol{x}_i^T\boldsymbol{\beta} + m_{i1} + \frac{m_{i2}}{1+m_{i2}^2}(Y_{i2} - \boldsymbol{x}_i^T\boldsymbol{\beta} - m_{i1}),\, \frac{\sigma^2}{1+m_{i2}^2}\right\}, & N_i \ge 2, \end{cases} \\ p(Y_{ij} \mid \text{—}) &\propto \mathcal{N}\left\{Y_{ij} \;\middle|\; \boldsymbol{x}_i^T\boldsymbol{\beta} + m_{i1} + \frac{m_{i2}}{1+m_{i2}^2}(Y_{i(j-1)} + Y_{i(j+1)} - 2\boldsymbol{x}_i^T\boldsymbol{\beta} - 2m_{i1}),\, \frac{\sigma^2}{1+m_{i2}^2}\right\}, \\ p(Y_{iN_i} \mid \text{—}) &\propto \mathcal{N}\{Y_{iN_i} \mid \boldsymbol{x}_i^T\boldsymbol{\beta} + m_{i1} + m_{i2}(Y_{i(N_i-1)} - \boldsymbol{x}_i^T\boldsymbol{\beta} - m_{i1}),\, \sigma^2\}, \quad N_i \ge 2; \end{aligned} \tag{S10}$$

for $T_{i(n_i+1)} > c_i$ and $T_{iN_i} \le S_i$. Let $R_{ij} = S_i - T_{iN_i} + e^{Y_{ij}} = S_i - \sum_{j^* \ne j} e^{Y_{ij^*}}$. Then, $e^{Y_{ij}}$ is bounded from above by $R_{ij}$ since $T_{iN_i} \le S_i$. Additionally, $e^{Y_{i(n_i+1)}}$ is bounded from below by $c_i - T_{in_i}$ since $T_{i(n_i+1)} > c_i$. Therefore, we can sample from (S10) with these truncations for $j = n_i + 1, \dots, N_i$ using the inverse transform method.

We sample $S_i$ from (S7) truncated to $S_i > c_i$ using the inverse transform method.

## S1.5 Dirichlet process parameters

As detailed in Section 1, the discreteness of the DP induces clustering of the individuals. Denote the random effects in the $h$th cluster by $(\boldsymbol{m}_h^*,\, \delta_h^*)$ and the cluster that individual $i$ belongs to by $s_i$. Then, $s_i = h$ if and only if $(\boldsymbol{m}_i,\, \delta_i) = (\boldsymbol{m}_h^*,\, \delta_h^*)$. To update $(\boldsymbol{m}_i,\, \delta_i)$ for $i = 1, \dots, L$, we update the cluster allocations $s_i$ and the cluster-specific parameters $(\boldsymbol{m}_h^*,\, \delta_h^*)$,

using Algorithm 8 from Neal (2000) with the algorithm-specific parameter $m = 2$. We choose this algorithm since independent sampling from the full conditional of $\boldsymbol{m}_h^*$, required for instance for Neal's Algorithm 2, is hard due to the intractability of the likelihood discussed in Section S1.1.

Neal's Algorithm 8 requires sampling of $(\boldsymbol{m}_h^*,\, \delta_h^*)$ that leaves its full conditional distribution invariant. We do this by first sampling $m_{h1}^*$, then $m_{h2}^*$ and lastly $\delta_h^*$ such that their respective full conditionals remain invariant. A derivation analogous to the one for (S5) yields the full conditional for $m_{h1}^*$. Specifically, we introduce $Y_{i1}^{m_{i1}} = Y_{i1} - \boldsymbol{x}_i^T\boldsymbol{\beta}$, $Y_{ij}^{m_{i1}} = \{Y_{ij} - \boldsymbol{x}_i^T\boldsymbol{\beta} - m_{i2}(Y_{i(j-1)} - \boldsymbol{x}_i^T\boldsymbol{\beta})\}/(1 - m_{i2})$ for $j = 2, \ldots, N_i$ and the $N_i \times N_i$ diagonal matrix $\boldsymbol{\Sigma}_{m_{i1}}$ with $\operatorname{diag}(\boldsymbol{\Sigma}_{m_{i1}}) = \sigma^2\,\{1,\,(1-m_{i2})^{-2},\,\ldots,\,(1-m_{i2})^{-2}\}^T$. Then,

$$p(m_{h1}^* \mid \text{—}) \propto \frac{\mathcal{N}(m_{h1}^* \mid \mu_{m_{h1}^*}^*,\, \Sigma_{m_{h1}^*}^*)}{\prod_{\{i \mid s_i = h\}} \Pr(T_{iN_i}^* \leq S_i^*)}, \tag{S11}$$

where $\mu_{m_{h1}^*}^* = \Sigma_{m_{h1}^*}^* \sum_{\{i|s_i=h\}} \mathbf{1}_{1\times N_i}\boldsymbol{\Sigma}_{m_{i1}}^{-1}\boldsymbol{Y}_i^{m_{i1}}$ and $\Sigma_{m_{h1}^*}^* = 1/\{1/\sigma_m^2 + \sum_{\{i|s_i=h\}} \operatorname{sum}(\boldsymbol{\Sigma}_{m_{i1}}^{-1})\}$ with $\operatorname{sum}(\boldsymbol{\Sigma}_{m_{i1}}^{-1}) = \{1 + (N_i - 1)(1 - m_{i2})^2\}/\sigma^2$.

Similarly for $m_{h2}^*$, we introduce $Y_{i(j-1)}^{m_{i2}} = (Y_{ij} - \boldsymbol{x}_i^T\boldsymbol{\beta} - m_{i1})/(Y_{i(j-1)} - \boldsymbol{x}_i^T\boldsymbol{\beta} - m_{i1})$ for $j = 2, \ldots, N_i$ and the $(N_i - 1)\times(N_i - 1)$ diagonal matrix $\boldsymbol{\Sigma}_{m_{i2}}$ with $(\boldsymbol{\Sigma}_{m_{i2}})_{jj} = \sigma^2/(Y_{ij} - \boldsymbol{x}_i^T\boldsymbol{\beta} - m_{i1})^2$ for $j = 1, \ldots, N_i - 1$. Then,

$$p(m_{h2}^* \mid \text{—}) \propto \frac{\mathcal{N}(m_{h2}^* \mid \mu_{m_{h2}^*}^*,\, \Sigma_{m_{h2}^*}^*)}{\prod_{\{i \mid s_i = h\}} \Pr(T_{iN_i}^* \leq S_i^*)}, \tag{S12}$$

where $\mu_{m_{h2}^*}^* = \Sigma_{m_{h2}^*}^* \sum_{\{i|s_i=h\}} \mathbf{1}_{1\times N_i}\boldsymbol{\Sigma}_{m_{i2}}^{-1}\boldsymbol{Y}_i^{m_{i2}}$ and $\Sigma_{m_{h2}^*}^* = 1/\{1/\sigma_m^2 + \sum_{\{i|s_i=h\}} \operatorname{sum}(\boldsymbol{\Sigma}_{m_{i2}}^{-1})\}$ with $\operatorname{sum}(\boldsymbol{\Sigma}_{m_{i2}}^{-1}) = \sum_{j=1}^{N_i-1}(Y_{ij} - \boldsymbol{x}_i^T\boldsymbol{\beta} - m_{i1})^2/\sigma^2$.

For $\delta_h^*$, a derivation similar to the one for (S8) yields

$$p(\delta_h^* \mid \text{—}) \propto \frac{\mathcal{N}(\delta_h^* \mid \mu_{\delta_h^*}^*,\, \Sigma_{\delta_h^*}^*)}{\prod_{\{i \mid s_i = h\}} \Pr(T_{iN_i}^* \leq S_i^*)} \tag{S13}$$

where $\mu_{\delta_h^*}^* = \Sigma_{\delta_h^*}^* \sum_{\{i|s_i=h\}}\{\log(S_i) - \boldsymbol{x}_i^T\boldsymbol{\gamma}\}/\eta^2$ and $\Sigma_{\delta_h^*}^* = 1/(1/\sigma_\delta^2 + |\{i \mid s_i = h\}|/\eta^2)$. Now, the update of $(\boldsymbol{m}_h^*,\, \delta_h^*)$ follows as slice sampling with (S11–S13) as target density for $h = 1, \ldots, K$ where $K$ is the number of clusters.

Equation 13 from Escobar and West (1995) provides the Gibbs update for the DP concentration parameter $M$: First, draw $\eta_M \sim \operatorname{Beta}(M + 1,\, L)$. Then, with probability $1/[1 + L\,\{b_M - \log(\eta_M)\}/(a_M + K - 1)]$ where $L$ denotes the number of individuals, draw $M \sim \operatorname{Gamma}\{a_M + K,\, b_M - \log(\eta_M)\}$. Otherwise, draw $M \sim \operatorname{Gamma}\{a_M + K - 1,\, b_M - \log(\eta_M)\}$.

## S1.6 Variance parameters, $r$ and $\lambda$

Recalling the prior and likelihood for $\sigma^2$ from Section 2.3 and (3), respectively, we obtain

$$p(\sigma^2 \mid \text{—}) \propto \frac{\text{Inv-Gamma}\{\sigma^2 \mid (\nu_{\sigma^2} + \sum_{i=1}^L N_i)/2,\, (\nu_{\sigma^2}\,\sigma_0^2 + \sum_{i=1}^L \|\boldsymbol{Y}_i - \boldsymbol{\mu}_i^{\sigma^2}\|^2)/2\}}{\prod_{i=1}^L \Pr(T_{iN_i}^* \leq S_i^*)}, \tag{S14}$$

where $\mu_{i1}^{\sigma^2} = \boldsymbol{x}_i^T\boldsymbol{\beta} + m_{i1}$ and $\mu_{ij}^{\sigma^2} = \boldsymbol{x}_i^T\boldsymbol{\beta} + m_{i1} + m_{i2}(Y_{i(j-1)} - \boldsymbol{x}_i^T\boldsymbol{\beta} - m_{i1})$ for $j = 2, \ldots, N_i$. Similarly for $\eta^2$, its prior from Section 2.3 and the likelihood in (S7) yield

$$p(\eta^2 \mid —) \propto \frac{\text{Inv-Gamma}\{\eta^2 \mid (\nu_{\eta^2} + L)/2,\ (\nu_{\eta^2}\,\eta_0^2 + \sum_{i=1}^L \{\log(S_i) - \boldsymbol{x}_i^T\boldsymbol{\gamma} - \delta_i\}^2)/2\}}{\prod_{i=1}^L \Pr(T_{iN_i}^* \leq S_i^*)}. \tag{S15}$$

Now, the Gibbs updates for $\sigma^2$ and $\eta^2$ follow as slice sampling with (S14) and (S15) as target density, respectively.

The full conditionals for $r$ and $\lambda$ follow, up to proportionality, from their gamma priors in Section 2.3 and the negative binomial likelihood from Section 2.2,

$$p(\boldsymbol{N} \mid r, \lambda) = \prod_{i=1}^L \frac{\Gamma(N_i + r)}{\Gamma(r) N_i!} p(r,\lambda)^{N_i}\{1 - p(r,\lambda)\}^r, \tag{S16}$$

where $\Gamma(\cdot)$ is the gamma function and $p(r,\lambda) = \lambda/(\lambda + r)$. The updates for $r$ and $\lambda$ follow then as slice sampling with these full conditionals.

# S2 Prior specification

For the application of our model to the AF data in Section S4, the hyperparameters of the prior distributions in Section 2.3 are chosen as follows. The hyperparameters of the priors on $\sigma^2$ and $\eta^2$ are such that their prior means equal 1 and their prior variances equal 100. Specifically,

$$\begin{aligned}
\mathrm{E}(\sigma^2) &= \frac{\nu_1\,\sigma_0^2/2}{\nu_1/2 - 1} = \frac{\nu_1\,\sigma_0^2}{\nu_1 - 2} = 1, \\
\mathrm{Var}(\sigma^2) &= \frac{\nu_1^2\,\sigma_0^4/4}{(\nu_1/2 - 1)^2\,(\nu_1/2 - 2)} = \frac{2\,\nu_1^2\,\sigma_0^4}{(\nu_1 - 2)^2\,(\nu_1 - 4)} = 100, \\
\mathrm{E}(\eta^2) &= \frac{\nu_2\,\eta_0^2/2}{\nu_2/2 - 1} = \frac{\nu_2\eta_0^2}{\nu_2 - 2} = 1, \\
\mathrm{Var}(\eta^2) &= \frac{\nu_2^2\,\eta_0^4/4}{(\nu_2/2 - 1)^2\,(\nu_2/2 - 2)} = \frac{2\,\nu_2^2\,\eta_0^4}{(\nu_2 - 2)^2\,(\nu_2 - 4)} = 100;
\end{aligned}$$

yields $\nu_1 = 4.02$, $\sigma_0^2 = 2.02/4.02$, $\nu_2 = 4.02$ and $\eta_0^2 = 2.02/4.02$. Similarly, the prior variances of the elements of the regression coefficients $\boldsymbol{\beta}$ and $\boldsymbol{\gamma}$ equal $\sigma_\beta^2 = \sigma_\gamma^2 = 100$. The hyperparameters related to the base measure $G_0$ of the DP prior are chosen as non-informative with $\sigma_\delta^2 = \sigma_m^2 = 100$. We choose an uninformative prior on the DP concentration parameter $M$ with $a_M = 2$ and $b_M = 1$. Finally, $a_r = b_r = a_\lambda = b_\lambda = 1$ specifies the priors for $r$ and $\lambda$.

# S3 Additional simulation studies

## S3.1 Prior sensitivity study

This section considers the effect of choosing different hyperparameters $a_\lambda$ and $b_\lambda$ on the posterior inference for the number of recurrent events $N_i$. Specifically, consider the simulated data from Section 3 where 90% of the individuals are censored. Then, we run the Gibbs sampler with $a_\lambda = \mu_\lambda^2$ and $b_\lambda = \mu_\lambda$, such that $E(\lambda) = \mu_\lambda$ and $\text{Var}(\lambda) = 1$ a priori, for $\mu_\lambda = 0.1, 1, 10$ with the remainder of the set-up being the same as in Section 3.

Figure S1 shows the posterior inference on $N_i$ analogously to Figure 1. The results do not vary notably across the different choices of prior mean $\mu_\lambda$.

## S3.2 Model misspecification

In Section 3, the data are simulated from the model in Section 2.2. Here, we consider data that are simulated from a different model. Specifically, we do not generate the survival times $S_i$ from a log-normal distribution as per (4) but instead from a Gompertz distribution with shape parameter 0.01 and scale parameter $\exp(-\boldsymbol{x}_i^T\boldsymbol{\gamma} - \delta_i)$. Then, $E(S_i \mid \boldsymbol{\gamma}, \delta_i, \eta^2) = \exp(\boldsymbol{x}_i^T\boldsymbol{\gamma} + \delta_i + 1.41)$. Under the log-normal distribution in (4), we have $E(S_i \mid \boldsymbol{\gamma}, \delta_i, \eta^2) = \exp(\boldsymbol{x}_i^T\boldsymbol{\gamma} + \delta_i + \eta^2/2)$, such that the regression coefficients $\boldsymbol{\gamma}$ retain their interpretation under the misspecification using the Gompertz distribution as data generation process. The remainder of the set-up is the same as in Section 3.

Figures S2 through S6 present the results analogously to Figures 1 through 5. Posterior inference appears robust to the misspecification with the credible intervals for $N_i$ mostly covering the true values (Figure S2) and the credible intervals for the regression coefficients all covering the true values (Figure S6). The posterior mode for the number of clusters is not equal to the true value of three in the absence of censored data (Figure S5). This is unsurprising as the Dirichlet process can accommodate any empirical distribution by adding further mixture components when necessary

## S3.3 Bias and mean squared error of the posterior means

To assess the bias and the mean squared error (MSE) of the posterior means of our method, we repeat the simulation of Section 3 eight times. Then, we estimate the bias as the difference between the average of the resulting eight posterior means and the parameter values from which the data were generated. We compute the MSE analogously.

Table S1 contains the results. For those parameters for which the bias or MSE varies notably with the censoring level, we consistently see that higher censoring results in larger bias and MSE.

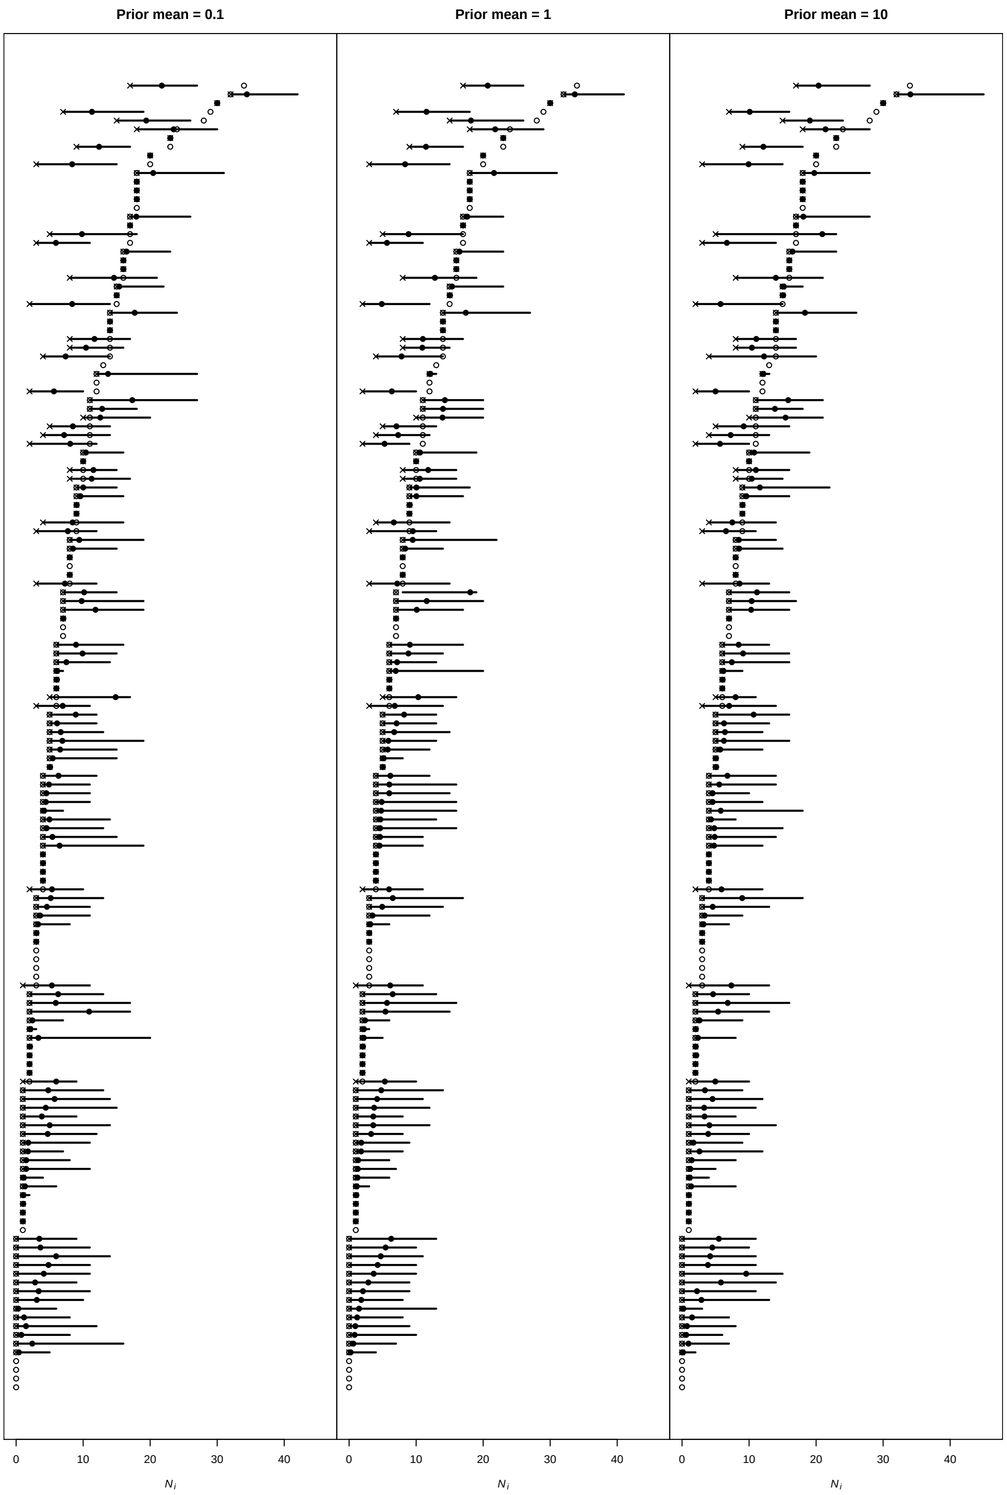


Figure S1: The number of gap times $N_i$ (circle) and, if applicable, their posterior means (dot) and 95% posterior credible intervals (lines) for each individual from our model fitted on the simulated data with 90% censoring and different prior means for $\lambda$. For censored individuals, the number of observed gap times $n_i$ is marked by '$\times$'.

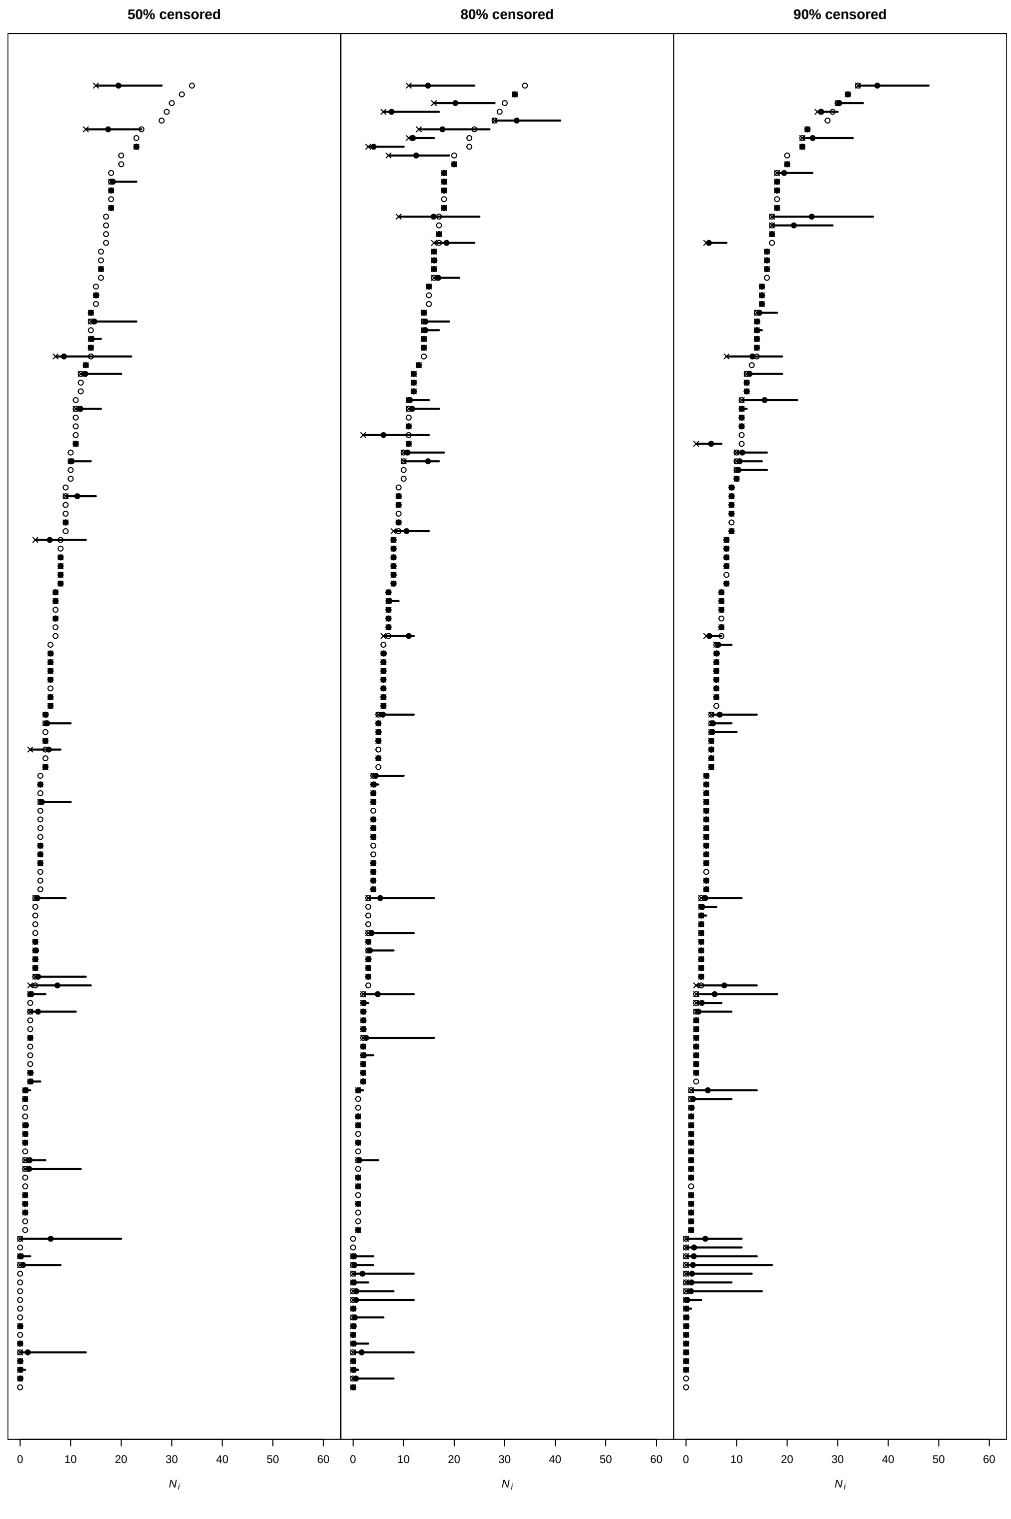


Figure S2: The number of gap times $N_i$ (circle) and, if applicable, their posterior means (dot) and 95% posterior credible intervals (lines) for each individual from our misspecified model fitted on the data simulated from a Gompertz distribution. For censored individuals, the number of observed gap times $n_i$ is marked by '×'.

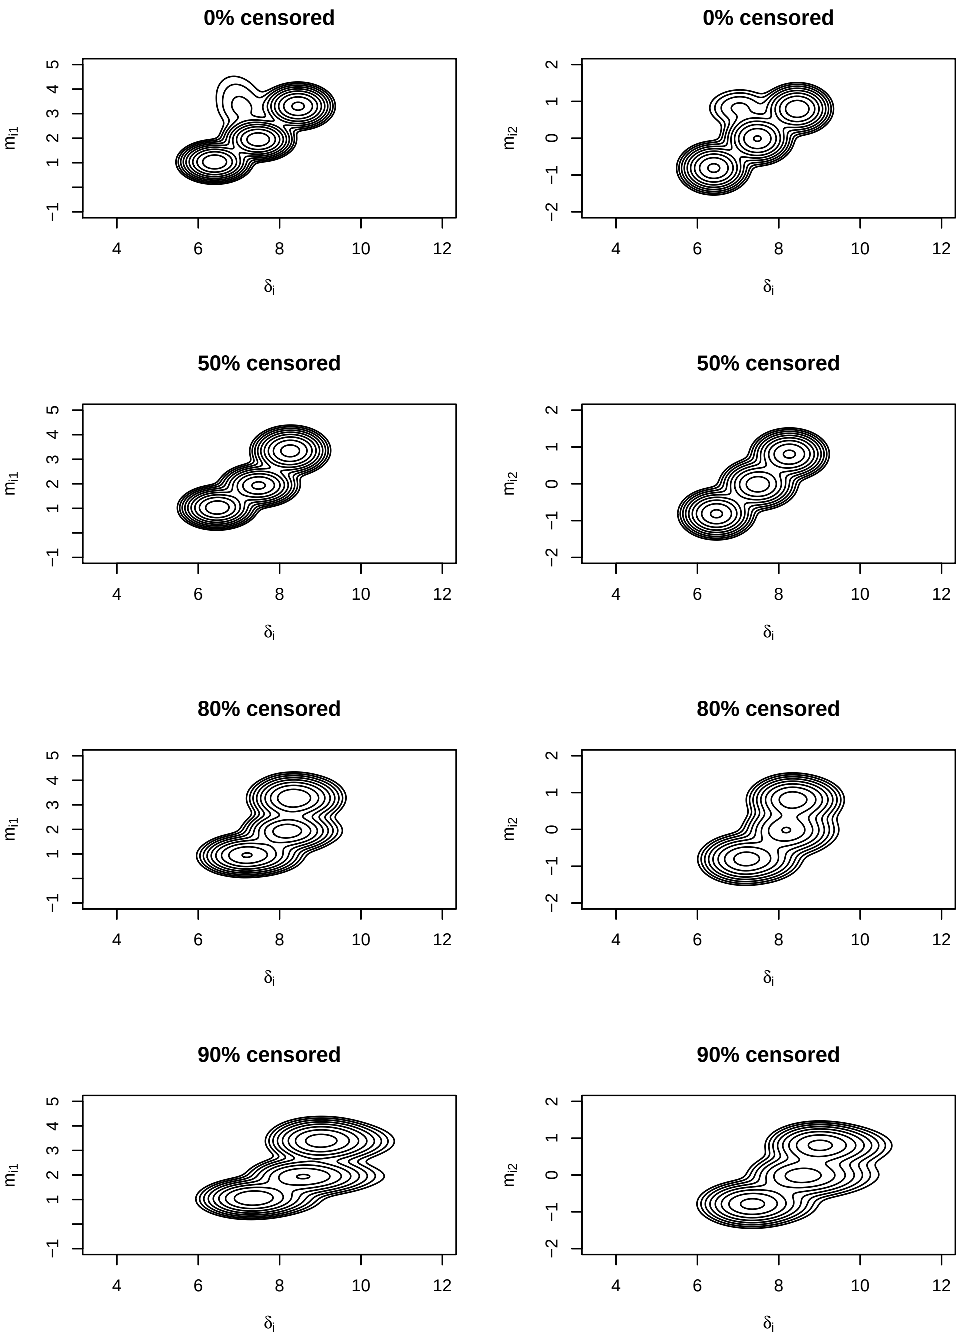


Figure S3: Contour plots of the log of the bivariate posterior predictive densities of $(m_{i1}, \delta_i)$ (left) and $(m_{i2}, \delta_i)$ (right) for a hypothetical new individual from the data simulated from a Gompertz distribution.

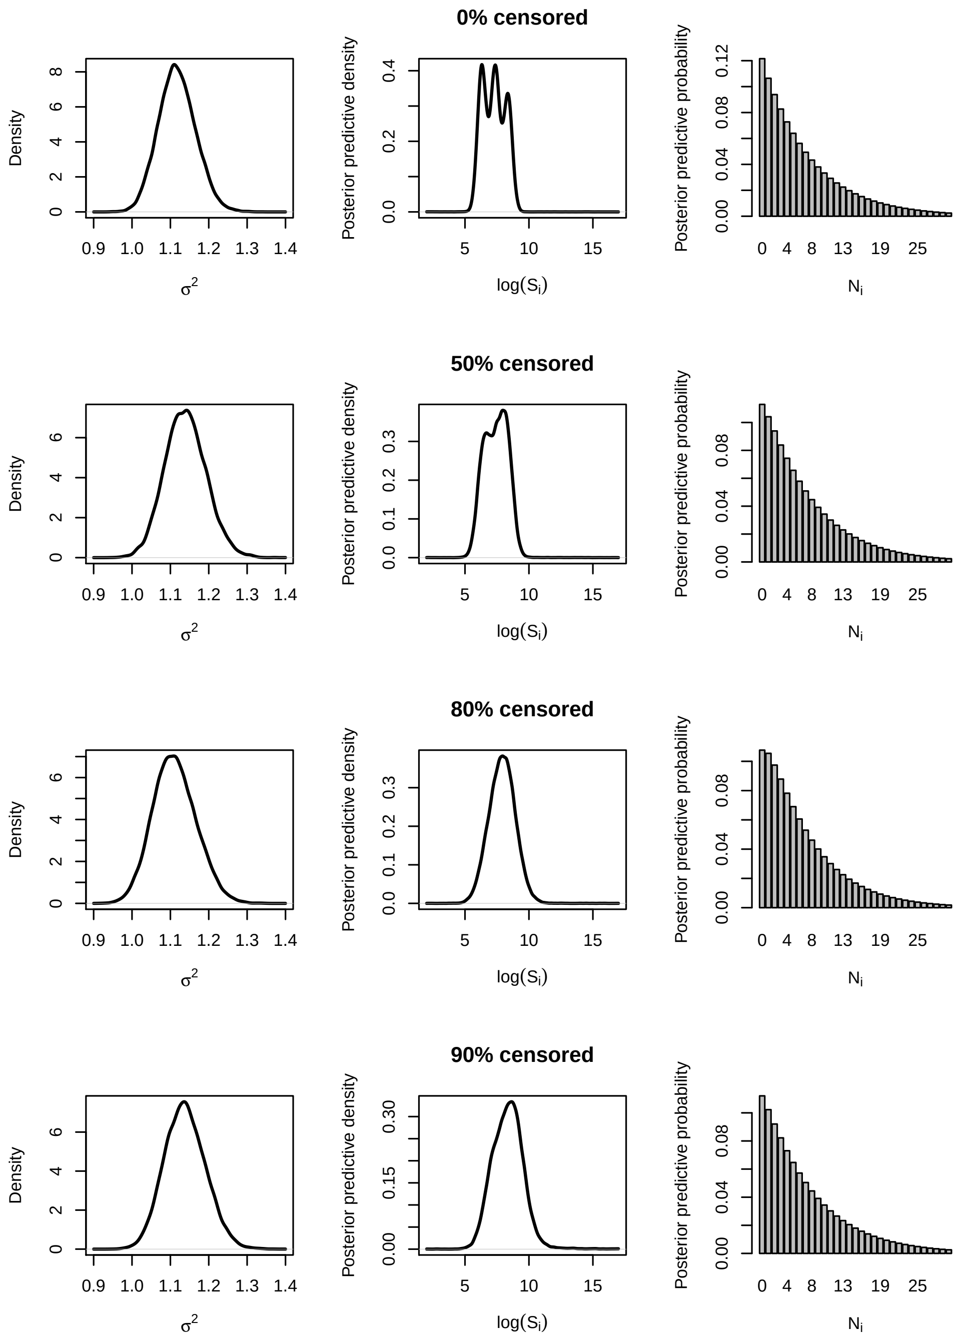


Figure S4: Posterior density for $\sigma^2$, and posterior predictive density for $\log(S_i)$ and posterior predictive probability mass function for $N_i$ for a hypothetical new patient with covariates equal to their sample medians from our misspecified model fitted on the data simulated from a Gompertz distribution.

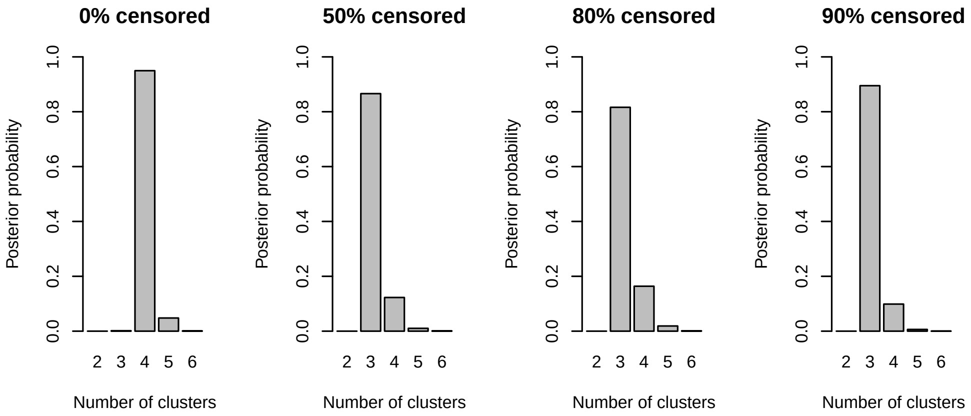


Figure S5: Posterior distribution of the number of clusters from our misspecified model fitted on the data simulated from a Gompertz distribution.

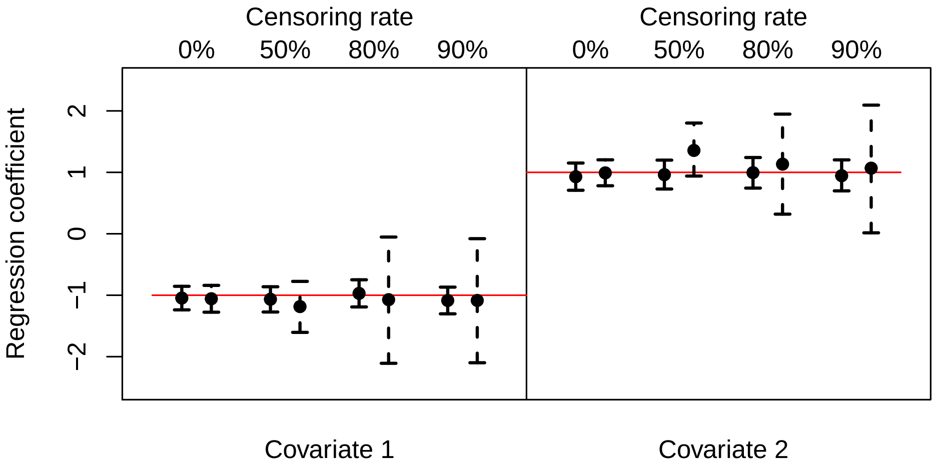


Figure S6: Posterior means (dot) and 95% marginal posterior credible intervals (lines) of the regression coefficients from our misspecified model fitted on the data simulated from a Gompertz distribution. The solid lines represent credible intervals for the regression coefficients $\boldsymbol{\beta}$ in (3) for the gap times model. The dashed lines correspond with the regression coefficients $\boldsymbol{\gamma}$ in (4) for the survival times. The horizontal line marks the true $\boldsymbol{\beta} = \boldsymbol{\gamma} = (-1, 1)^T$ from which the data were simulated.

Table S1: Bias (root mean squared error) of posterior means from our model fitted on simulated data.

| Parameter | $\beta_1$ | $\beta_2$ | $\gamma_1$ | $\gamma_2$ |
|---|---|---|---|---|
| 0% censored | 0.16 (0.38) | -0.13 (0.36) | 0.00066 (0.20) | -0.22 (0.45) |
| 50% censored | 0.17 (0.38) | -0.13 (0.36) | -0.02 (0.23) | -0.15 (0.46) |
| 80% censored | 0.089 (0.25) | -0.12 (0.24) | -0.32 (0.69) | 0.088 (0.79) |
| 90% censored | 0.071 (0.17) | -0.025 (0.16) | 0.18 (1.05) | -0.25 (0.70) |

| Parameter | $m^*_{11}$ | $m^*_{21}$ | $m^*_{31}$ |
|---|---|---|---|
| 0% censored | 0.20 (0.21) | 0.047 (0.073) | -0.29 (0.31) |
| 50% censored | 0.33 (0.33) | 0.12 (0.14) | -0.25 (0.29) |
| 80% censored | 0.44 (0.44) | 0.23 (0.25) | -0.21 (0.24) |
| 90% censored | 0.45 (0.46) | 0.18 (0.26) | -0.26 (0.29) |

| Parameter | $m^*_{12}$ | $m^*_{22}$ | $m^*_{32}$ |
|---|---|---|---|
| 0% censored | 0.18 (0.19) | 0.036 (0.071) | -0.22 (0.22) |
| 50% censored | 0.27 (0.28) | 0.077 (0.11) | -0.25 (0.26) |
| 80% censored | 0.33 (0.33) | 0.11 (0.13) | -0.26 (0.26) |
| 90% censored | 0.35 (0.35) | 0.11 (0.13) | -0.28 (0.28) |

| Parameter | $\delta^*_1$ | $\delta^*_2$ | $\delta^*_3$ |
|---|---|---|---|
| 0% censored | 0.37 (0.51) | 0.14 (0.26) | -0.17 (0.24) |
| 50% censored | 0.84 (0.93) | 0.57 (0.67) | 0.18 (0.38) |
| 80% censored | 1.65 (1.74) | 1.59 (1.67) | 1.22 (1.30) |
| 90% censored | 2.92 (3.11) | 2.59 (2.64) | 2.97 (3.17) |

# S4 Application to atrial fibrillation data

## S4.1 Background

In addition to the colorectal cancer data considered in Section 4, we apply our model to data on atrial fibrillation (AF) described in Schroder et al. (2019b) AF is the most common serious cardiac arrhythmia with more than 33 million cases worldwide, increasing rapidly with five million new cases per year (Chung et al., 2020). It is characterized by an irregular and often high heart rate where the heart's upper chambers beat out of sync with its lower chambers. AF causes substantial morbidity and mortality, for instance due to heart failure and stroke. It places a high burden on health care systems, constituting 2.4% of the United Kingdom's National Health Service budget in 2000 (Thrall et al., 2006).

AF is often a chronic condition that requires repeated treatment. The goal of these treatments is to reduce the rate of AF episodes, as an increased number of episodes is associated with complications such as stroke (Munger et al., 2014). Thus, there is dependence between recurrence and survival, which our model is able to capture. Additionally, more frequent AF events are associated with an increase in the rate of episodes going forward (Wijffels et al., 1995). This points to temporal dependence in the AF recurrence process, as captured in our model by (3).

A variety of treatments exist. These include prophylactic anti-arrhythmic medication and cardioversion (Schroder et al., 2019b). Anti-arrhythmic medication aims to reduce the rate and duration of AF episodes. Cardioversion aims to restore the heart rhythm when it is abnormal, that is while someone is experiencing an AF episode. Cardioversion is either electrical, using direct currents, or pharmacologic. Electrical cardioversion takes place in a hospital. AF diagnosis usually requires an electrocardiogram (ECG).

The condition of AF can be categorized into three subtypes: paroxysmal, persistent and permanent (January et al., 2014). Episodes of paroxysmal AF terminate spontaneously without treatment. In contrast, persistent AF is when the episode only ends due to an intervention. Lastly, AF is permanent when the patient and clinician decide to no longer attempt to restore the heart rhythm. Additionally, AF episodes are either symptomatic or asymptomatic. Symptoms of AF include palpitations and chest pain.

As for many other chronic diseases, clinical interest lies in both the final outcome (death or survival time) and the dynamics of the process itself, since it determines the subsequent quality of the patient's life (Thrall et al., 2006). From an economic and healthcare planning perspective, there is great interest in reducing rehospitalization for AF. In fact, a better understanding of both death and non-fatal clinical events could lead to improved prognosis and assessment of the impact and costs of AF by health providers. It is, therefore, of paramount importance to develop a comprehensive model for disease management, mortality and associated clinical event histories, which also accounts for the significant interindividual variability in disease course as it is typical of chronic diseases and biological events, and can infer the number of rehospitalizations as it closely relates to economic cost.

Table S2: Frequency table of the number of observed gap times $n_i$ in the AF data.

| $n_i$ | 0 | 1 | 2 | 3 | 4 | 5 | 6 | 7 | 8 | 9 | 10 | 11 | 12 | 13 | 14 | 15 | 16 |
|---|---|---|---|---|---|---|---|---|---|---|---|---|---|---|---|---|---|
| Frequency | 29 | 11 | 9 | 9 | 3 | 3 | 9 | 4 | 2 | 0 | 2 | 1 | 0 | 1 | 0 | 0 | 1 |

## S4.2 Data description and analysis

The data (Schroder et al., 2019a) consist of hospitalizations from January 1, 2008 to March 1, 2014 at the Department of Cardiology at University Hospital Copenhagen, Hvidovre, Denmark (Schroder et al., 2019b). The primary reason of all hospitalizations is symptomatic AF. Some include cardioversion treatment. AF is confirmed by ECG. We consider $L = 84$ patients that experience at least one hospitalization due to non-permanent AF. This first hospitalization represents the origin of a patient's recurrence process such that $T_{i0} = 0$ for all $i$. Using an event time as origin is standard practice in models for gap times (Cook and Lawless, 2007), though a different origin, if available, could be chosen to also include individuals who experience no events. Consequently, $n_i$ represents the number of observed gap times between subsequent hospitalizations due to non-permanent AF. Patients experience between zero and 16 *re*hospitalizations each and $\sum_{i=1}^{L} n_i = 241$ in aggregate. Table S2 shows how they are distributed across patients. Gap times are defined as the difference between successive hospitalizations and, as such, capture both the length of stay in the hospital and the time between discharge and the next hospitalization.

The main clinical outcome of interest is deterioration to permanent AF or death. We therefore define the survival time $S_i$ as the time to permanent AF or death. The survival times of 68 out of the 84 recurrence processes are censored due to the follow-up ending on March 1, 2014, resulting in unobserved total number of gap times $N_i$.

Patient characteristics are determined at the first hospitalization. They are 1) age; and the binary variables 2) gender; whether 3) AF is paroxysmal or persistent; and whether the patient has 4) hypertension; 5) heart disease; or 6) is on anti-arrhythmic medication. Here, heart disease includes heart failure, heart valve disease and ischemic heart disease. These variables form the subject-specific 6-dimensional covariate vector $\boldsymbol{x}_i$, with $q = 6$. Being older or female, hypertension, and heart disease are known to be associated with more severe AF (January et al., 2014). Anti-arrhythmic medication aims to prevent and ameliorate the reoccurrence of AF. We standardize the age in $\boldsymbol{x}_i$. Table S3, and Figures S7 and S8 summarize the patient characteristics, and the gap and survival times.

We use the same priors, from Section S2, and set-up of the Gibbs sampler as the simulation study in Section 3.

## S4.3 Posterior inference

The posterior inference is summarized in Figures S9 through S13 analogously to the colorectal cancer application in Section 4.

Figure S9 summarizes the posterior distribution of the total number of gap times $N_i$ for each patient. The posterior means for the censored $N_i$ are generally in line with the observed

Table S3: Summary statistics of the AF data and the posterior from our model. The averages and standard deviations of posterior means are taken across patients and recurrent events. $S_i$ is recorded in days and $Y_{ij}$ in log days.

| | |
|---|---|
| Number of patients | 841 |
| Proportion censored | 81% |
| Average uncensored $N_i$ | 1.75 (2.15) |
| Average posterior mean of $N_i$ (SD) | 3.99 (3.72) |
| Average uncensored $Y_{ij}$ (SD) | 4.17 (1.61) |
| Average posterior mean of $Y_{ij}$ (SD) | 4.72 (1.26) |
| Average uncensored $\log(S_i)$ (SD) | 5.72 (1.25) |
| Average posterior mean of $\log(S_i)$ (SD) | 11.6 (3.27) |
| Average age (SD) | 58.2 (12.2) |
| Proportion female | 32% |
| Proportion with paroxysmal AF | 15% |
| Proportion with hypertension | 46% |
| Proportion with heart disease | 20% |
| Proportion on anti-arrhythmic medication | 12 % |

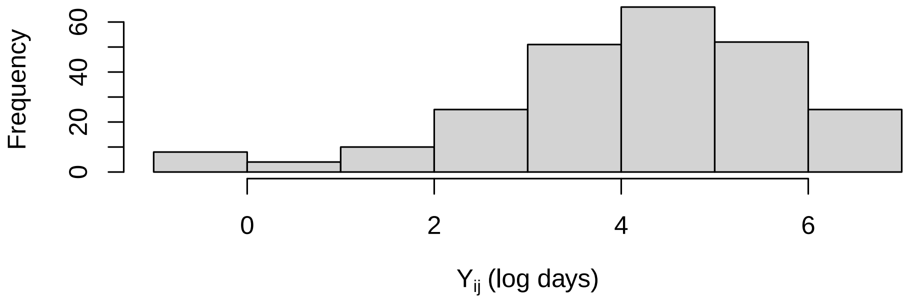


Figure S7: Histogram of the 241 observed log gap times $Y_{ij}$ in the AF data.

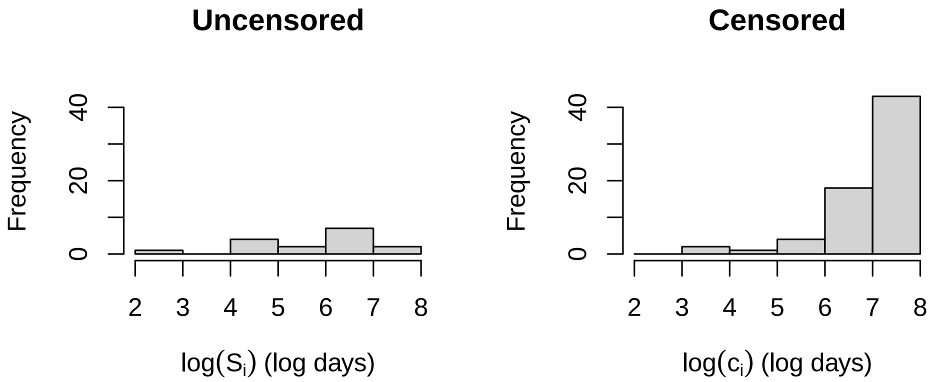


Figure S8: Histograms of the log of the 16 observed survival times $S_i$ (left) and the 68 censoring times (right) in the AF data. If the survival time $S_i$ is observed, then $c_i = S_i$.

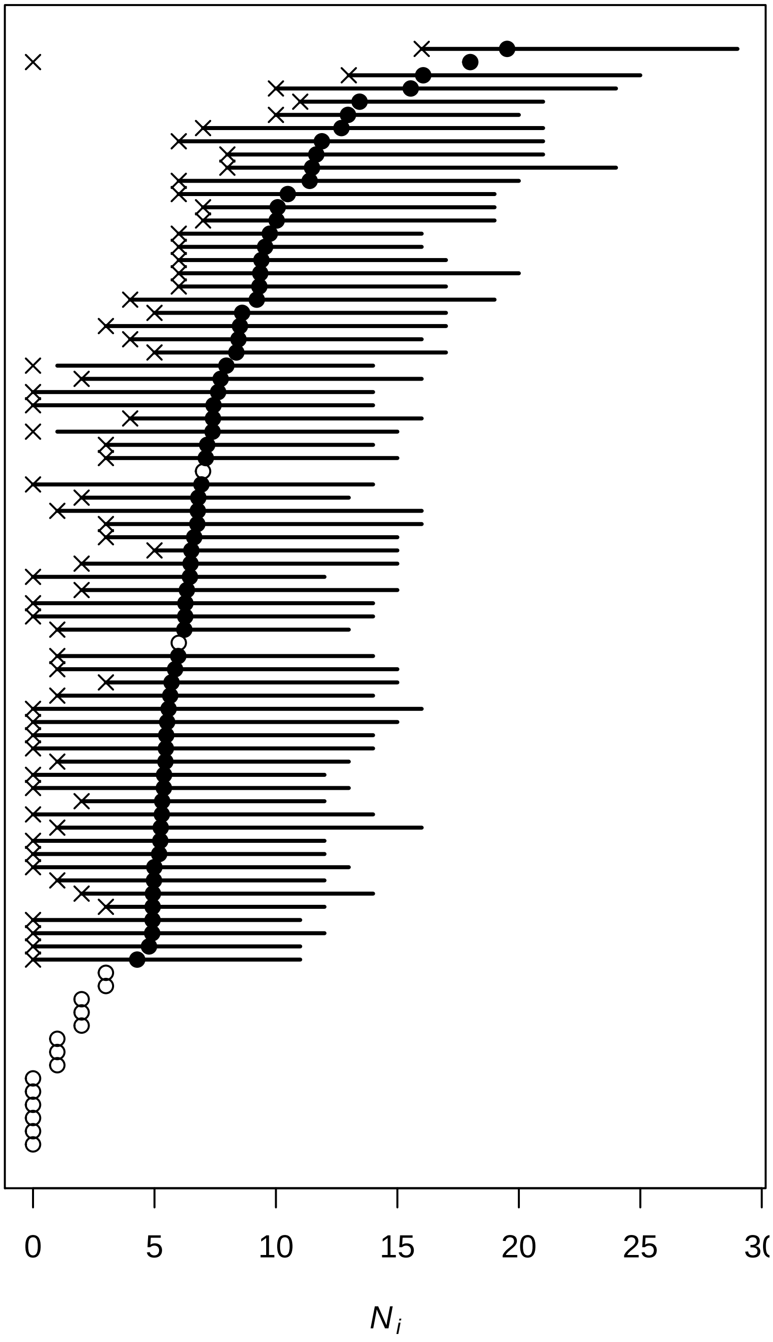


Figure S9: The number of gap times $N_i$ (circle) if observed and otherwise their posterior means (dot) and 95% posterior credible intervals (lines) for each patient from our model fitted on the AF data. For censored patients, the number of observed gap times $n_i$ is marked by '×'.

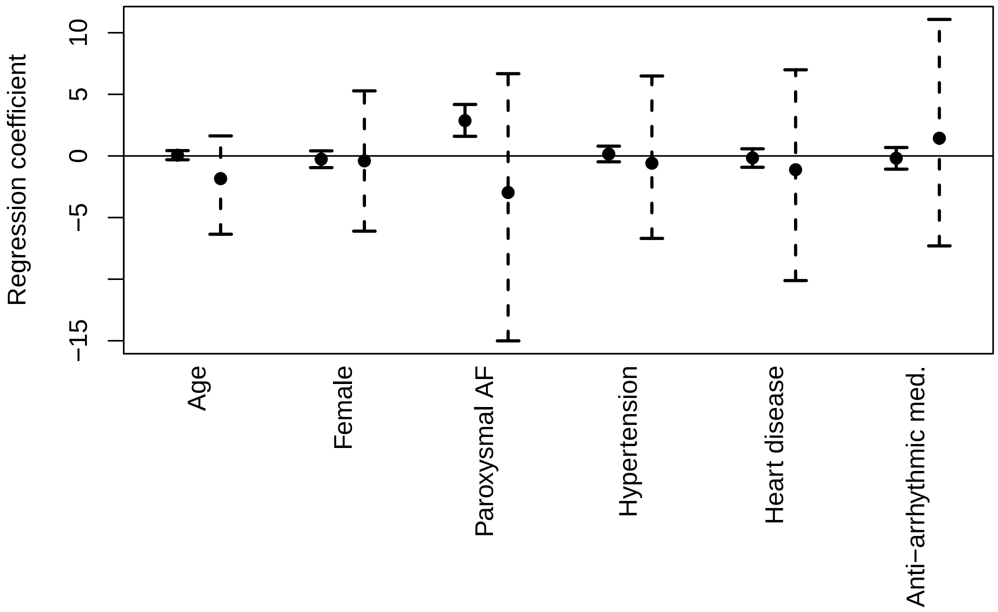


Figure S10: Posterior means (dot) and 95% marginal posterior credible intervals (lines) of the regression coefficients from our model fitted on the AF data. The solid lines represent credible intervals for the regression coefficients $\boldsymbol{\beta}$ in (3) for the gap times model. The dashed lines correspond with the regression coefficients $\boldsymbol{\gamma}$ in (4) for the survival times.

$N_i$. The unobserved $N_i$ are sometimes inferred to be larger than the largest observed $N_i$. After all, the largest observed $N_i$ equals seven while the number of observed gap times $n_i$ is 16 for one patient. This is expected since patients with longer survival times $S_i$ are both more likely to have a higher number of gap times $N_i$ and to be censored due to end of study.

Figure S10 shows no evident effect of any of the covariates as the corresponding 95% credible intervals include 0, except for the interval for the effect of paroxysmal AF on gap times which excludes zero. This is in line with the analysis of these data described in Schroder et al. (2019b) The relatively small sample size of $L = 84$ might be the reason that we do not find strong effects, even though most of these covariates are risk factors for AF.

Figure S11 shows that the posterior marginals of $(m_{i1}, \delta_i)$ and $(m_{i2}, \delta_i)$ are unimodal. The cluster allocation that minimizes the posterior expectation of Binder's(Binder, 1978) loss function confirms this with all subjects clustered together. Finally, Figure S13 also has the posterior mode at one cluster.

## S4.4 Comparison with other models

We consider that same model comparisons for the AF data as we did for the colorectal cancer data in Section 5. The results are presented in Figures S14 through S16, and Tables S4 and S5.

When fitting the Cox proportional hazard model, we include a patient's log mean gap

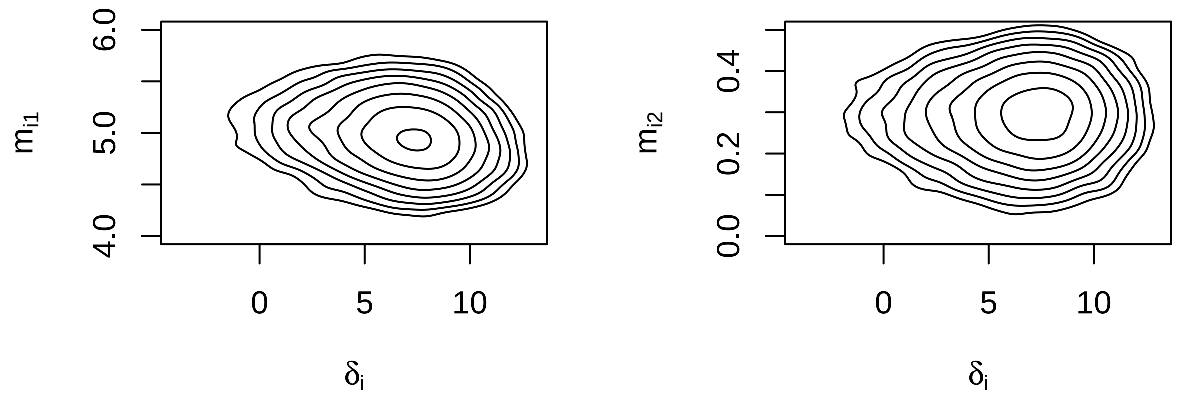


Figure S11: Contour plots of the log of the bivariate posterior predictive densities of $(m_{i1}, \delta_i)$ (left) and $(m_{i2}, \delta_i)$ (right) for a hypothetical new patient from the AF data.

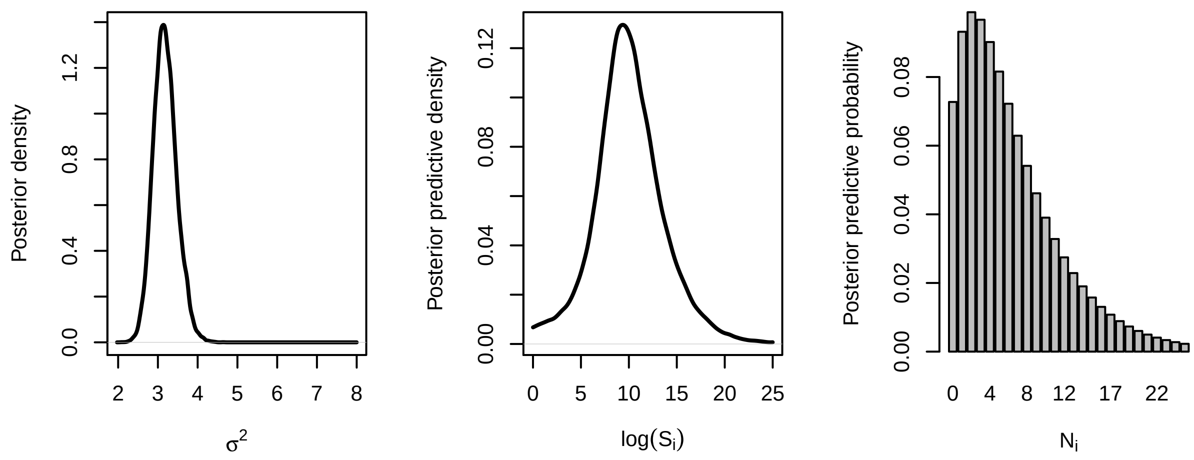


Figure S12: Posterior density for $\sigma^2$, and posterior predictive density for $\log(S_i)$ and posterior predictive probability mass function for $N_i$ for a hypothetical new patient with binary covariates equal to their sample mode and with age equal to the sample median from our model fitted on the AF data.

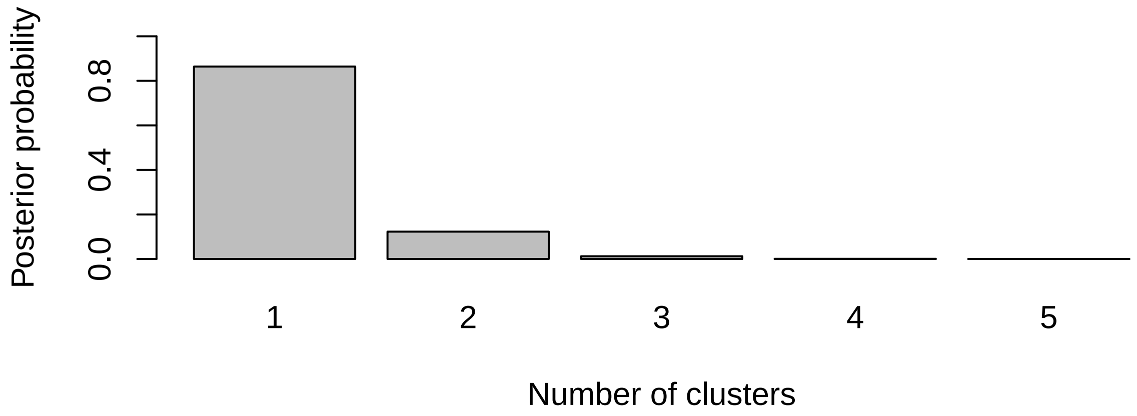


Figure S13: Posterior distribution of the number of clusters from our model fitted on the AF data.

Table S4: Regression coefficients from the Cox proportional hazards model fitted on the AF data.

| Covariate | Hazard ratio | 95% CI |
|---|---|---|
| Age | 2.06 | (0.95, 4.47) |
| Female | 1.33 | (0.30, 5.92) |
| Paroxysmal AF | 3.55 | (0.36, 35.4) |
| Hypertension | 1.02 | (0.22, 4.83) |
| Heart disease | 1.12 | (0.19, 6.52) |
| Antiarrhythmic medication | 0.50 | (0.06, 4.55) |
| Log mean gap time | 1.22 | (0.73, 2.05) |

time in the covariate vector $\boldsymbol{z}_i$ in addition to the six covariates included in $\boldsymbol{x}_i$ described in Section S4.2. As a result, the 29 individuals with no observed gap times are excluded. Table S4 shows the covariate effects on survival from the Cox proportional hazards model. They agree with the inference for $\boldsymbol{\gamma}$ from our model in Figure S10 in that they do not exhibit a significant effect.

To fit the joint frailty model (Rondeau et al., 2007) to the AF data, we drop hypertension from $\boldsymbol{x}_i$ due to convergence issues when using all covariates. The comparison of the joint frailty model results in Table S5 with our results in Figure S10 shows that both models obtain similar results and do not detect an association for most of the covariates while agreeing that paroxysmal AF reduces the rehospitalization rate. The models disagree on the effect of age on rehospitalization and survival, where the joint frailty model finds a statistically significant effect. Finally, the estimate of $\rho$ is 0.007 with a standard error of 0.001. This suggests heterogeneity between patients that is not explained by the covariates even though our model detected only a single cluster.

The Bayesian semi-parametric model from Paulon et al. (2018) yields conclusions that are largely consistent with those from our model. In particular, the posterior distributions on the coefficients in Figure S14 closely mimic our results in Figure S10. Also, the posterior on $\psi$ in (5) concentrates between 1.5 and 3.5 per Figure S15. This parameter captures the strength of the relationship between gap and survival times. Thus, the time between hospitalizations and survival have a positive association. This is consistent with the dependence implied by the truncation $T_{iN_i} \leq S_i$ in our model. Lastly, the posterior on the number of clusters for this model and our model vary slightly, with the mode at one clusters for our model in Figure S13 while Figure S16 has the mode at four. This is not surprising as discussed in Section 5.3.

# References


Aalen, O. O. and Husebye, E. (1991) Statistical analysis of repeated events forming renewal processes. *Statistics in Medicine*, **10**, 1227–1240.

Asmussen, S., Goffard, P.-O. and Laub, P. J. (2019) Orthonormal polynomial expansions and

Table S5: Regression coefficients from the joint frailty model fitted on the AF data.

| Rehospitalization | | |
|---|---|---|
| Covariate | Hazard ratio | $p$-value |
| Age | 1.01 | 0.04 |
| Female | 0.90 | 0.46 |
| Paroxysmal AF | 0.59 | 0.03 |
| Heart disease | 0.93 | 0.64 |
| Antiarrhythmic medication | 0.73 | 0.07 |
| **Mortality** | | |
| Covariate | Hazard ratio | $p$-value |
| Age | 1.10 | 0.04 |
| Female | 4.22 | 0.10 |
| Paroxysmal AF | 1.68 | 0.59 |
| Heart disease | 2.03 | 0.37 |
| Antiarrhythmic medication | 1.81 | 0.52 |

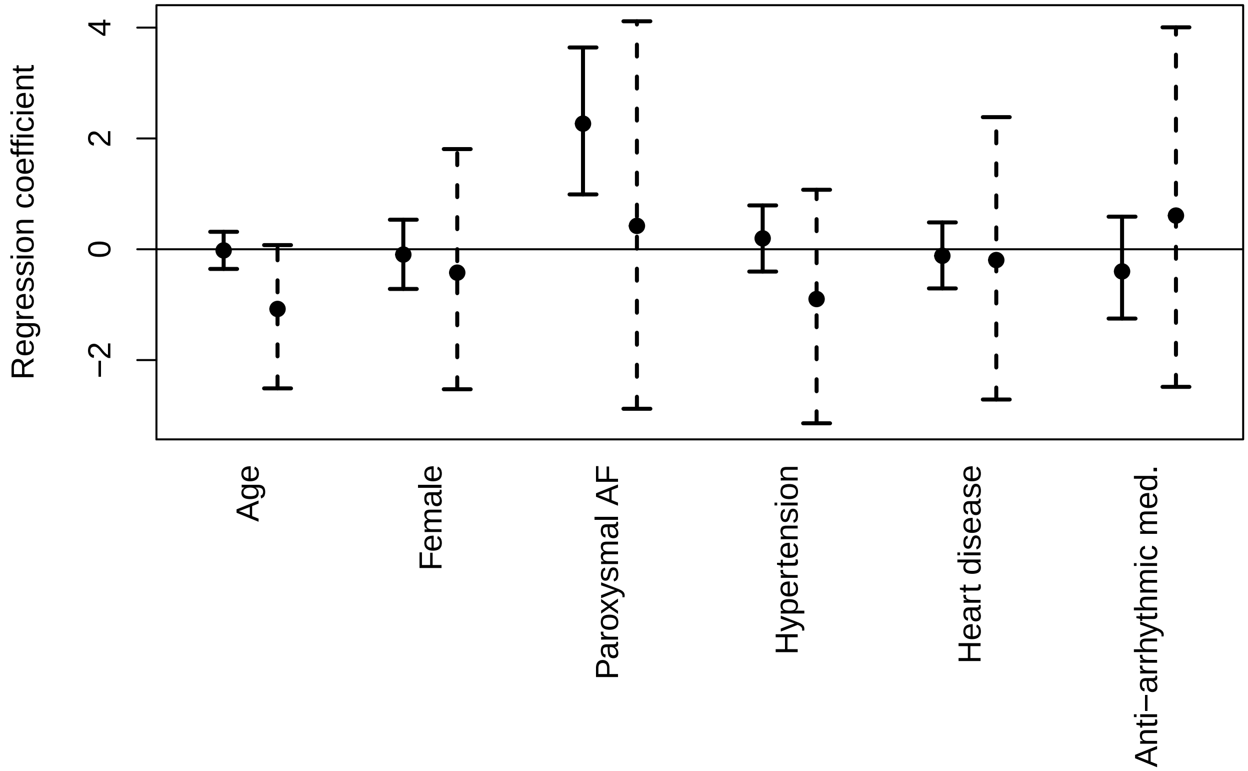


Figure S14: Posterior means (dot) and 95% marginal posterior credible intervals (lines) of the regression coefficients from the model in Paulon et al. (2018) fitted on the AF data. The solid lines represent credible intervals for the regression coefficients $\boldsymbol{\beta}$ in the gap times model. The dashed lines correspond to the regression coefficients $\boldsymbol{\gamma}$ in (5) for the survival times.

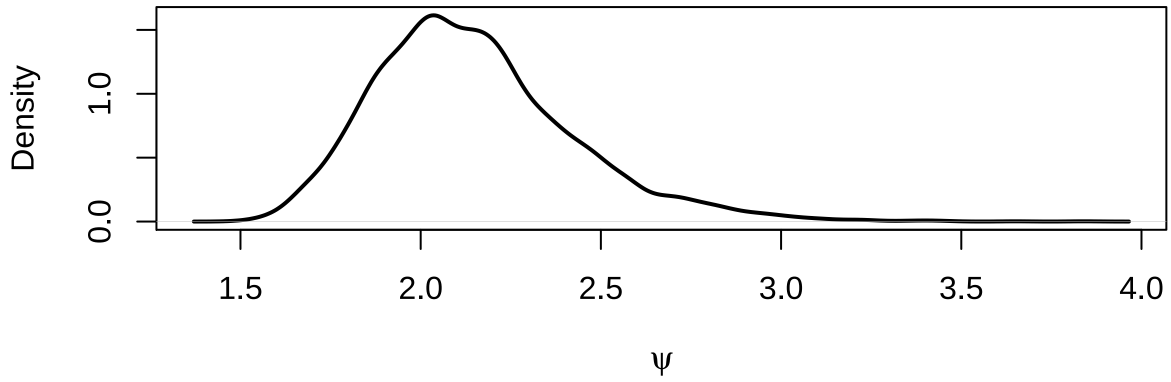


Figure S15: Posterior density for $\psi$ in (5) from the model in Paulon et al. (2018) fitted on the AF data.

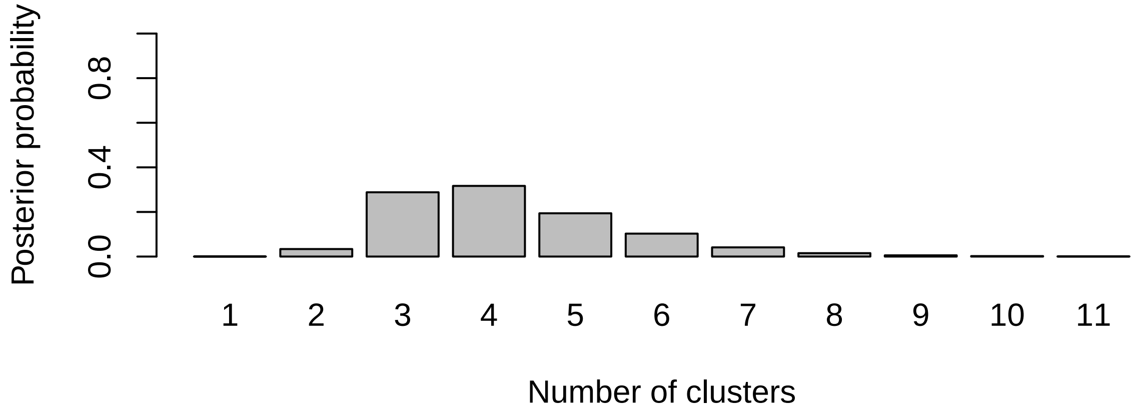


Figure S16: Posterior distribution of the number of clusters from the model from Paulon et al. (2018) fitted on the AF data.

lognormal sum densities. In *Risk and Stochastics*, 127–150. World Scientific.

Asmussen, S., Jensen, J. L. and Rojas-Nandayapa, L. (2016) Exponential family techniques for the lognormal left tail. *Scandinavian Journal of Statistics*, **43**, 774–787.

Binder, D. A. (1978) Bayesian cluster analysis. *Biometrika*, **65**, 31–38.

Botev, Z. I., Salomone, R. and Mackinlay, D. (2019) Fast and accurate computation of the distribution of sums of dependent log-normals. *Annals of Operations Research*, **280**, 19–46.

Chung, M. K., Eckhardt, L. L., Chen, L. Y., Ahmed, H. M., Gopinathannair, R., Joglar, J. A., Noseworthy, P. A., Pack, Q. R., Sanders, P. and and, K. M. T. (2020) Lifestyle and risk factor modification for reduction of atrial fibrillation: A scientific statement from the american heart association. *Circulation*, **141**.

Cook, R. J. and Lawless, J. F. (2007) *The statistical analysis of recurrent events*. Springer, New York.

Escobar, M. D. and West, M. (1995) Bayesian density estimation and inference using mixtures. *Journal of the American Statistical Association*, **90**, 577–588.

Fenton, L. (1960) The sum of log-normal probability distributions in scatter transmission systems. *IEEE Transactions on Communications*, **8**, 57–67.

Green, P. J. (1995) Reversible jump Markov chain Monte Carlo computation and Bayesian model determination. *Biometrika*, **82**, 711–732.

Halliwell, L. J. (2015) The lognormal random multivariate. *Casualty Actuarial Society E-Forum*, **Spring 2015**, 1–5.

January, C. T., Wann, L. S., Alpert, J. S., Calkins, H., Cigarroa, J. E., Cleveland, J. C., Conti, J. B., Ellinor, P. T., Ezekowitz, M. D., Field, M. E., Murray, K. T., Sacco, R. L., Stevenson, W. G., Tchou, P. J., Tracy, C. M. and Yancy, C. W. (2014) 2014 AHA/ACC/HRS guideline for the management of patients with atrial fibrillation. *Circulation*, **130**.

Munger, T. M., Wu, L.-Q. and Shen, W. K. (2014) Atrial fibrillation. *Journal of Biomedical Research*, **28**, 1–17.

Neal, R. M. (2000) Markov chain sampling methods for Dirichlet process mixture models. *Journal of Computational and Graphical Statistics*, **9**, 249–265.

Paulon, G., De Iorio, M., Guglielmi, A. and Ieva, F. (2018) Joint modeling of recurrent events and survival: A Bayesian non-parametric approach. *Biostatistics*. Kxy026.

Rondeau, V., Mathoulin-Pelissier, S., Jacqmin-Gadda, H., Brouste, V. and Soubeyran, P. (2007) Joint frailty models for recurring events and death using maximum penalized likelihood estimation: Application on cancer events. *Biostatistics*, **8**, 708–721.

Schroder, J., Bouaziz, O., Agner, B. R., Martinussen, T., Madsen, P. L., Li, D. and Dixen, U. (2019a) Full anonymized dataset used for statistical analysis. *figshare, doi:10.1371/journal.pone.0217983.s001.*

— (2019b) Recurrent event survival analysis predicts future risk of hospitalization in patients with paroxysmal and persistent atrial fibrillation. *PLOS ONE*, **14**, e0217983.

Tallarita, M., De Iorio, M., Guglielmi, A. and Malone-Lee, J. (2020) Bayesian autoregressive frailty models for inference in recurrent events. *The International Journal of Biostatistics*, **16**, 1–18.

Thrall, G., Lane, D., Carroll, D. and Lip, G. Y. (2006) Quality of life in patients with atrial fibrillation: A systematic review. *The American Journal of Medicine*, **119**, 448.e1–448.e19.

Waagepetersen, R. and Sorensen, D. (2001) A tutorial on reversible jump MCMC with a view toward applications in QTL-mapping. *International Statistical Review*, **69**, 49–61.

Wijffels, M. C., Kirchhof, C. J., Dorland, R. and Allessie, M. A. (1995) Atrial fibrillation begets atrial fibrillation. *Circulation*, **92**, 1954–1968.

Table S6: Regression coefficients from the Cox proportional hazards model fitted on the colorectal cancer data.

| Covariate | Hazard ratio | 95% CI |
|---|---|---|
| Chemotherapy | 1.56 | (0.96, 2.54) |
| Female | 0.55 | (0.33, 0.93) |
| Stage C | 2.91 | (1.40, 6.04) |
| Stage D | 11.5 | (5.58, 23.5) |
| Log mean gap time | 0.88 | (0.74, 1.04) |

Table S7: Regression coefficients from the joint frailty model fitted on the colorectal cancer data.

| Rehospitalization | | |
|---|---|---|
| Covariate | Hazard ratio | $p$-value |
| Chemotherapy | 0.86 | 0.30 |
| Female | 0.60 | 0.00 |
| Stage C | 1.53 | 0.01 |
| Stage D | 4.27 | 0.00 |
| Mortality | | |
| Covariate | Hazard ratio | $p$-value |
| Chemotherapy | 2.70 | 0.00 |
| Female | 0.76 | 0.24 |
| Stage C | 4.91 | 0.00 |
| Stage D | 52.8 | 0.00 |

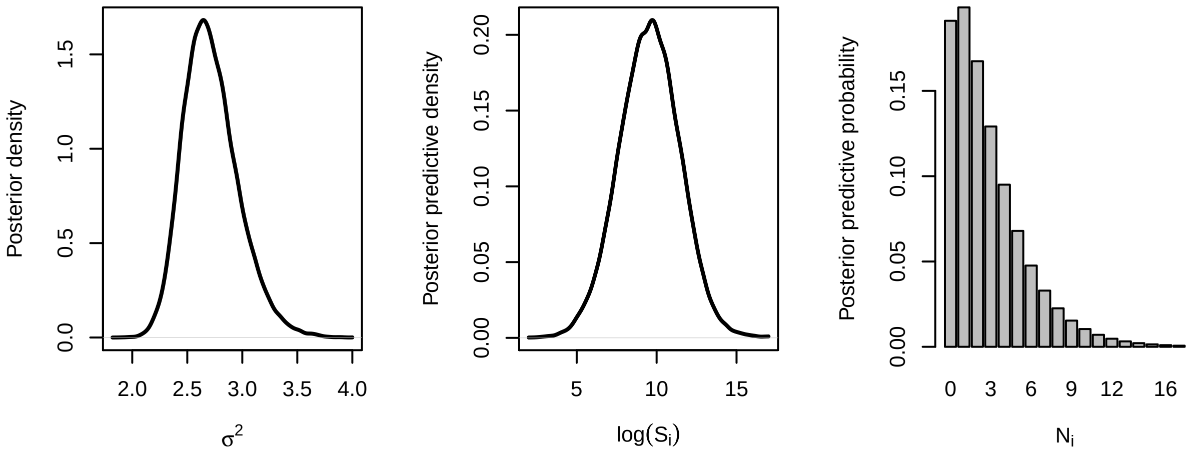


Figure S17: Posterior density for $\sigma^2$, and posterior predictive density for $\log(S_i)$ and posterior predictive probability mass function for $N_i$ for a hypothetical new patient with covariates equal to their sample mode from our model fitted on the colorectal cancer data.

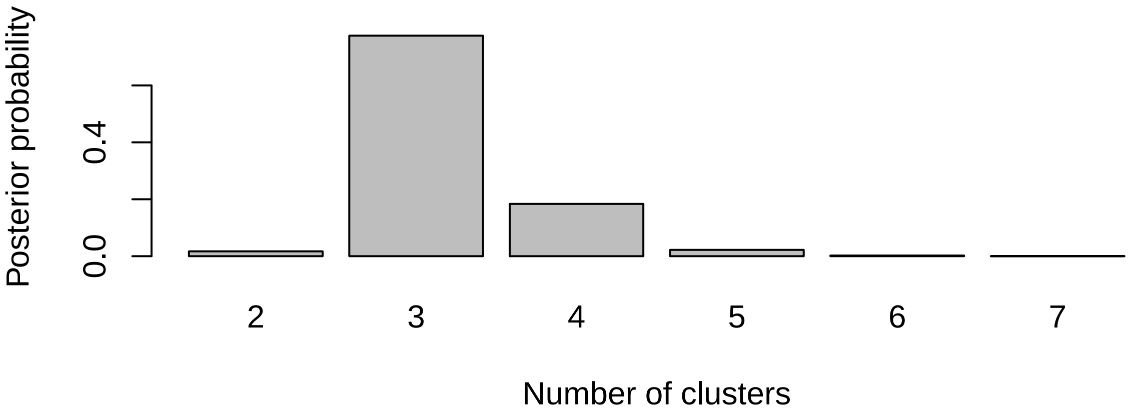


Figure S18: Posterior distribution of the number of clusters from our model fitted on the colorectal cancer data.

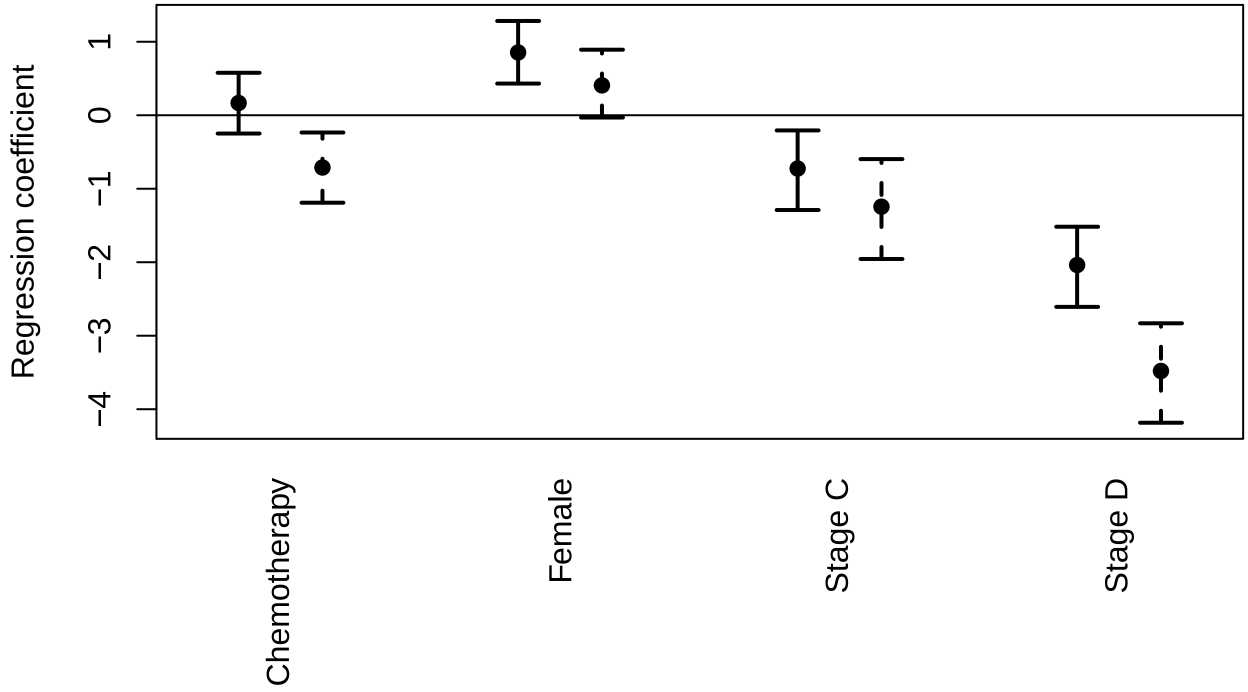


Figure S19: Posterior means (dot) and 95% marginal posterior credible intervals (lines) of the regression coefficients from the model in Paulon et al. (2018) fitted on the colorectal cancer data. The solid lines represent credible intervals for the regression coefficients $\boldsymbol{\beta}$ in the gap times model. The dashed lines correspond to the regression coefficients $\boldsymbol{\gamma}$ in (5) for the survival times.

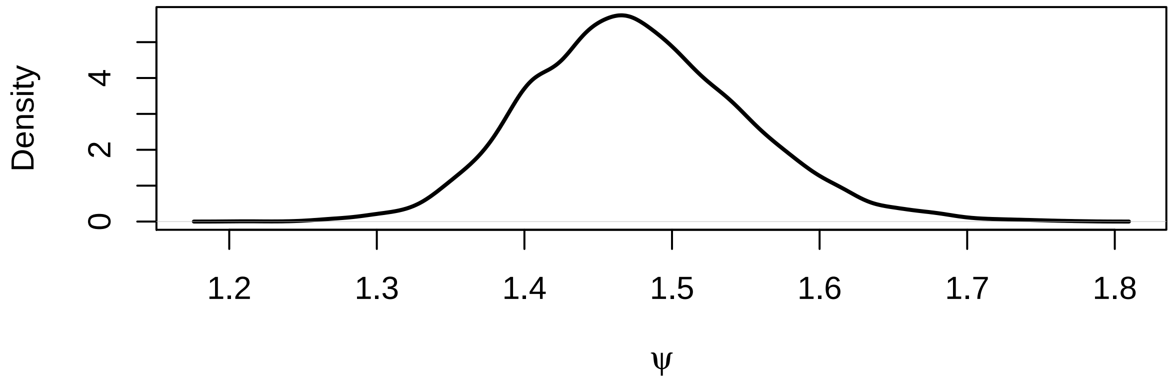


Figure S20: Posterior density for $\psi$ in (5) from the model in Paulon et al. (2018) fitted on the colorectal cancer data.

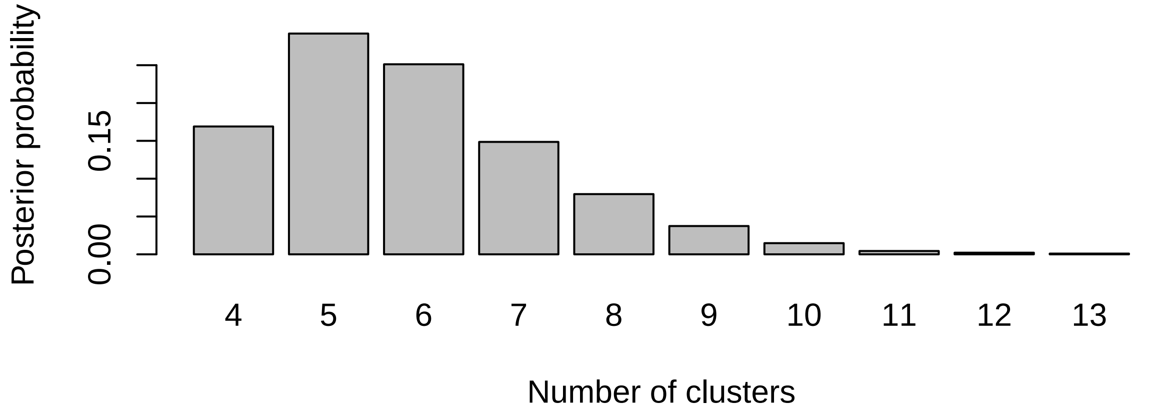


Figure S21: Posterior distribution of the number of clusters from the model from Paulon et al. (2018) fitted on the colorectal cancer data.
